# Supplementary material for: Critical Hyper-Parameters: No Random, No Cry
Source: arXiv:1706.03200 source file (2017-06-10)
Supplement: Supplementary file 1 [file appendix_endtoend.tex]

\section{End to end real-scale xps with LDS}\label{endtoendapp}
\def\longversion{1}
Mathematics above have shown positive results for LDS (rates in Theorems 1 and 2), recommendations (Theorem 3: variables should be ranked) and hints (Theorem 4: LDS outperform grids by far when a small set of variables are critical, as discussed in \cite{BergtraBengio}) as well as negative results (Theorems 5 and 6\ifthenelse{\longversion=0}{\ in the SM}{}: no LDS using countably many random bits can be consistent and LDS with random shift is consistent but does not have RFL). We have also seen negative results for most existing methods, except stratified sampling which, as in numerical integration, has no counter-example (Theorem 7\ifthenelse{\longversion=0}{\ in the SM}{}).
Toy xps confirmed everything. They also supported S-SH, among other tested LDS and design of experiments methods, for one-shot optimization.
There are however things that mathematics and toy xps above did not quantify: the importance in real-world settings and the impact of the distinction test/train/validation. This section provides experimental results in this direction, in particular on S-SH (chosen among our one-shot optimization methods because it performed best on artificial settings); compared mainly to the classical random search (see SM for other end-to-end comparisons).

\ifthenelse{\longversion=1}{
	\subsection{Datasets}}{{\bf{Datasets.}}}
\ifthenelse{\longversion=0}{
	We use the well known PTB\cite{ptb}, both at the byte and the word levels; we also use UB-PTB, which is PTB after random permutation of blocks of 200 lines - blocks are moved even between train/validation/test sets, so that there is no systematic bias between validation/test/train. We also use various toy datasets (anbn, ABNA, and more sophisticated hierarchical vocabularies) fully described in the SM.
In all cases, the loss functions are in bits-per-byte. 

	}{
Penn Treebank (PTB\cite{ptb}) is a well known language modeling testbed; we use it both at the level of bytes and at the level of words.
We also use Unbiased PTB (UB-PTB), our own variant in which train/test/valid are permuted in an i.i.d manner, by blocks of 200 lines, so that there is no 
systematic distribution shift between train/valid/test; a detailed description is beyond the scope of this paper and we plan to release this dataset publicly.

We also use various toy datasets.
Our toy datasets are indexed with one string (AN or ANBN or .N or others, detailed below) and 4 numbers.
For the toy dataset $C$, the 4 numbers are the vocabulary size (the number of letters),
maximum word size ($n$ or $N$), vocabulary growth and depth - unless specified otherwise, vocabulary growth is 10
and depth is 3.
	 There are also four parameters for ANBN, AN, .N and anbn; but the two last parameters are different: they are ``fixed size'' (True for fixed size, False otherwise) and ``size gaps'' (impact of size gaps equal to True detailed below). For example, toy(anbn,26,10,0,1) means that n is randomly drawn between 1 and 10, and that there are size gaps; whereas toy(anbn,26,10,1,0) means that n is fixed equal to 10 and there is no size gap. 
\begin{itemize}
	\item AN is a toy dataset with, as word, a single letter randomly drawn (once for each sequence)
  and repeated a fixed number of times (same number of times for different sequences, but different letter).
  For examples, the first sequence might be ``qqqqqq qqqqqq qqqqqq'' and the second one ``pppppp pppppp pppppp''.

	\item The ``ANBN'' testbed is made of words built by concatenating N copies of a given randomly drawn letter, followed by N copies of another randomly drawn letter.
The words are repeated until the end of the sequence. For different sequences, we have different letters, but the same number N.
	\item In the ``ABNA'' dataset, a word is one letter (randomly drawn, termed A), then N copies of another letter (randomly drawn and termed B),
  and then the first letter again.

	\item We also use the ``.N'' testbed, where the ``language'' to be modelled is made of sequences, each of them containing only one word (made of $N$ randomly independently drawn letters) repeated until the end
of the sequence. The first sequence might be ``bridereix bridereix bridereix'' and the second sequence ``dunlepale dunlepale dunlepale''.
	\item We also have ``anbn'' as a testbed: compared to ANBN, the number of letters vary for each word in a same sequence, and the letters vary even inside a sequence.
  The first sequence might be ``aaabbb ddddcccc db''.
  
	\item Finally, we use the ``C'' testbed, in which there are typically 26 letters (i.e. the vocabulary size is 26 unless stated otherwise), words are randomly drawn combinations of letters and there 
exists $V\times26$ words of e.g. 10 (word size) letters; and there exists $V^2\times 26$ groups (we might say ``sentences'') of 10 words, where $V$ is the ``vocabulary growth'';
there are 3 levels (letters, words, groups of words) when the depth is $3$. For example $toy(C,26,10,7,3)$ contains $26$ letters, 26$\times$7 words of length $10$,
and 26$\times 7^2$ groups of $10$ words. 

\end{itemize}

For each sequence of these artificial datasets, the word size N is randomly chosen uniformly between 1 and the maximum word size, except when fixed size is 1 - in which case the word size is always the maximum word size.

If size gaps is equal to True, then the test sizes used in test and validation
are guaranteed to not have been seen in training; 4 word sizes are randomly chosen for valid and for test, and the other 16 are used in training. There are
10 000 training sequences, 1000 validation sequences, 1000 test sequences. Each sequence is made of 50 words, except for C for which a sequence is one group of the maximum level.

In all toy sequences, letters which are not predictable given the type of sequence have a weight 0 (i.e. are not taken into account when computing the loss).
In all cases, the loss functions are in bits-per-byte.
}
\ifthenelse{\longversion=1}{
\subsection{Experimental setup}
}{{\bf{Experimental setup.}}}
%We compare various sampling algorithms, a.k.a. one-shot optimization algorithm, for various models and various datasets. As pointed out in \cite{BergtraBengio} in which such xps on LDS are suggested but not performed, a key issue is that we work on samplings, so that statistical results are obtained by comparing many samples instead of one run - a computationally expensive task, so we carefully designed the criteria, prior to the runs.
\ifthenelse{\longversion=1}{
	\subsubsection{Stacked LSTM}}{}
Most of our xps consider stacked LSTM, with an output module. Experiments are in language modeling, applied to real or toy datasets as described above.
\ifthenelse{\longversion=1}{
\subsubsection{Parameters in leaky cells}}{}
In some xps, we consider LSTM\cite{Schmidthuber} augmented with leak \cite{leaky} in the $c$ part of the LSTM. We do this because it is a recent implementation in
our platform for which the correct tuning was unknown.
The $i^{th}$ coordinate of the state $c_t$ of the LSTM at time $t$, is replaced with $(\tilde c_t)_i = \tau_i (\tilde c_{t-1})_i + (1-\tau_i) (c_t)_i$. With $\tau_i=0$,
there is no leak, whereas $\tau_i=1$ means that the leaky cells have constant values.
The coefficients of the leaky cells are randomly drawn according to $\tau_i = sigmoid(\mu+\sigma \N)$, where $\N$ is a standard Gaussian, $sigmoid(x)=1/(1+exp(-x))$,
and $\mu$ and $\sigma$ are HPs.
\ifthenelse{\longversion=1}{
	\subsubsection{Ordering variables}}{}
Section \ref{ordering} recommended to use most important variables first; however, it is not that easy to know which variables are the most important.
In particular, after being tuned to reasonable values for the family of problems at hand, a critical variable becomes far less critical.
In all our xps, the learning
rate and the maximum gradient norm (in gradient clipping) are first and second
respectively, others are arbitrarily ranked.
\begin{figure}          % NOTINICML
		\center          % NOTINICML
			\includegraphics[width=.3\linewidth]{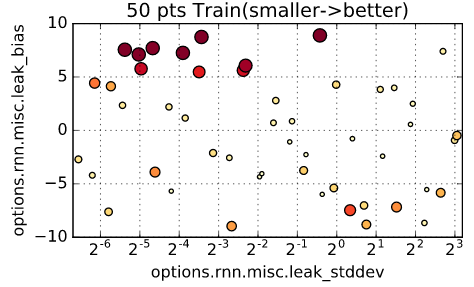}          % NOTINICML
				\includegraphics[width=.3\linewidth]{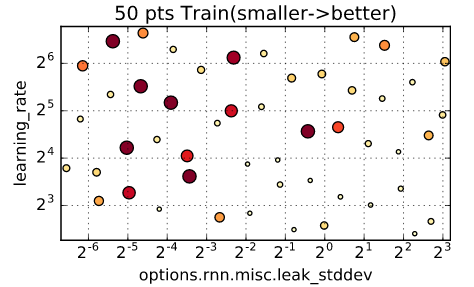}          % NOTINICML
					\includegraphics[width=.3\linewidth]{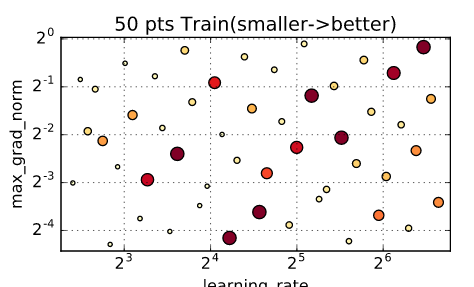}          % NOTINICML
					\ifthenelse{\longversion=1}{          % NOTINICML
						\caption{\label{qrleak}Various views of the sampling in the leaky context. Bigger/darker points correspond to worse training errors.  The learning rate and maximum gradient norm have the most regular sampling, consistently with the fact that they are ranked first in the list (first variables are more quasirandomized than last ones) - but, from the size of points, it looks like leaky parameters are actually more important than gradient norm and clipping norm - so the positive results in this testcase (Table \ref{leaky} and Fig. \ref{leakyfig}) show that LDS can be beneficial in spite of a wrong ranking of variables (Theorem 4).}}{          % NOTINICML
						\caption{\label{qrleak}Various views of the sampling in the leaky context. Bigger/darker points correspond to worse training errors.  The learning rate and maximum gradient norm have the most regular sampling, consistently with the fact that they are ranked first in the list (first variables are more quasirandomized than last ones) - but, from the size of points, it looks like leaky parameters are actually more important than gradient norm and clipping norm - so the positive results in this testcase show that LDS can be beneficial in spite of a wrong ranking of variables (Theorem 4).}}          % NOTINICML
\end{figure}          % NOTINICML
\ifthenelse{\longversion=1}{
\subsubsection{Dune-quantiles as a cross-dataset measure of performance}
The criterion is the average Dune-score $z_i$ for method $i$, designed as follows:
\begin{itemize}
\item let $r_{i,j}$ be the performance of method $i$ on problem $j$ (measured loss on test set);
\item let $q_{i,j}$ be the normalized rank of method $i$ on problem $j$ (i.e. the number of methods which perform better than $i$ in test on $j$, divided by the number of methods minus $1$);
\item let $s_{i,j}$ be the normalized score of method $i$ on problem $j$ (i.e. the loss in test, minus the minimum of all losses on problem $j$, divided by the difference between the maximum and the minimum loss on problem $j$);
\item the dune-quantile is then $z_{i,j} = \frac12(q_{i,j} + s_{i,j})$; and the overall Dune-score of a method $i$ is $z_i$, average of the $z_{i,j}$.
\end{itemize}
This criterion was designed prior to the study. $q_{i,j}$ was designed for being stable in front to rescaling of data and robust to outliers (extreme bad scores). $s_{i,j}$ was designed also for being stable in front of rescaling, and also for reducing the impact of very small differences.

\subsubsection{Logarithmic sampling}}{}
Ranges of HPs are sampled logarithmically when the whole range is positive and contains at least one value $\leq 0.1$. Other HPs are sampled linearly.
\ifthenelse{\longversion=1}{
	\subsubsection{Statistical significance \& speed-up}}{}\label{suapp}
\ifthenelse{\longversion=1}{
We present several forms of results: p-values (aimed at validating LDS over a large campaign of xps over several datasets and several budgets), starred p-values (aimed at validating one specific method, against random instances only, for one specific budget value), doubly-starred p-values (for validating one method, against all other methods, for one specific budget).

All p-values are computed with Fisher's exact test\cite{fisher71}.}{}
\ifthenelse{\longversion=0}{
We here  present speed-ups defined as follows.
}{We now present detailed protocols for evaluating p-values.

%TODO OMG we have to make the paragraph below super clear which is a challenge :-)
	{\bf{(Unstarred) p-values: significance for the specified LDS methods (for all LDS methods in the considered xp, if no LDS is specified).  }}
	For each budget, methods are ranked per dune-quantile, and the test uses the different budgets as independent values for performing Fisher's exact test. The statistic is the frequency at which the best result from LDS outperforms the best result from non-LDS methods, for the null assumption that all methods are equally likely to perform best.
\begin{itemize}
\item p-value $<$ 0.05 is a significant win for the considered LDS;
\item when random methods perform better we consider the p-value of the opposite null hypothesis and
      use a prefix ``opp'': opp-p-value $<$ 0.05 is therefore a significant win for random.
\end{itemize}
When NaiveDOE is present, the p-value is for quasirandom methods vs both random methods and naiveDoe.
For each budget value, the statistic is the Dune-quantile previously defined, averaged over all datasets.
Then the p-value is the probability under the null assumption that a LDS is ranked first as many times as in the data.

{\bf{Starred-p-values: significance for one LDS method compared to random methods and for one single budget value. }} For starred p-values, the result is based on the frequency, over the datasets,
   with which the considered LDS performed better than all random methods; this is computed for each LDS method separately.
   SH refers to Scrambled Hammersley. The prefix "S-" (e.g. S-SH) means that a random shift is applied. We do not apply Dune-quantiles for starred-p-values, because starred-p-values consider a single budget so that we have to use the different datasets as independent values for Fisher's exact test.

{\bf{Doubly-starred-p-values: significance for one LDS method compared to all other tested methods, for one single budget value.}} The doubly starred p-value is the probability, under null assumption, that this LDS method outperforms all other tested methods with at least the frequency observed in the data (same null hypothesis: all methods are equally likely to perform best). The difference with starred-p-values is that we compare to all other methods (i.e. not only to random methods).

{\bf{Speed-up:}} for additional readability we also present speed-ups.
}
The speed-up is the additional budget that would be necessary, under null assumption, so that the frequency of ``LDS wins'' is the observed one.
For example, a first pure random sampler wins with probability $2/3$ against a second random sampler if it has a twice larger budget - therefore, if LDS wins with probability $2/3$ against random with a same budget, we will say that the speed-up is +100\%;
and if one LDS instance wins with probability $3/5$ against 2 random instances with the same budget, we define the speed-up as +200\% (i.e. it is equivalent to 3 random instances).
We point out that this speed-up, in a fully parallel setting, is not really a speed-up - it's about reaching the same performance with a better sampling as if we had used more machines and a naive sampling.
Two additional speed-ups can easily be defined:
\begin{itemize}
	\item Average speed-up: the additional budget such that ``LDS has the same expected rank among the group (LDS + random instances) as if it was equivalent to a random instance equipped with this additional budget''.
	\item Robustness speed-up: the additional budget such that ``LDS has the same frequency of being ranked last among the group (LDS+random instances) as if etc''.
\end{itemize}
%These two additional speed-ups are referred to as ``average-speedup'' and ``robustness-speedup'' respectively.
\ifthenelse{\longversion=0}{
The detailed statistical analysis is presented in the SM.
	}{
		\subsection{Experimental results}}
\ifthenelse{\longversion=0}{
	{\bf{Experimental results.}}
%%%%%%%%%%% ICML BEGIN %%%%%%%%%%%%%%%%%%%%%%%%%%%%%%%%%%%%%%%%%%%%%%%%%%%%%%%
	The notation ``a:b:c'' refers to $\{a,a+b,a+2b,\dots,c\}$ and $a:b$ refers to $a:1:b$. ``*'' refers to datasets PTB words, PTB bytes, and 4 toy sequences.
	** refers to 6 toy datasets.
	*** refers to PTB bytes, PTB words, and 12 toy datasets.
	``Tuned'' refers to ranges $[0.02,1]\times[0.02,1]\times[0.5,30]$ for the weight init scale $\times$ the maximum gradient norm $\times$ the learning rate.
	``Untuned'' refers to ranges $[0.02,1]\times[0.002,100]\times [0.001,3000]$ for the same HP.
	``Half-tuned'' refers to ranges $[0.02,1]\times[0.006,30]\times[0.1,200]$.
	``Leaky'' refers to ranges $[-9,9]\times [0.01,10]\times[0.05,1]\times[0.02,1]\times[5,100]$ for the average of the leak parameters distribution$\times$ the standard deviation of this distribution $\times$ the maximum gradient norm $\times$ the weight init scale $\times$ the learning rate.
	In all cases, the learning rate and gradient clipping norm are used as first HP; in the leaky context, the most important variables are the two leaky parameters and they are arbitrarily ranked {\em{after}} these two HP.
	See SM for P-values. Our results are overviewed in Table \ref{main}.
	\begin{table}
		\scriptsize
	\begin{tabular}{|c|c|c|c|c|}
		\hline
		Setting       & Budgets              &                 & Average     &  Robustness \\
		                  &                            & Speed-up & speed-up   &  speed-up     \\
				  \hline
				  \hline
				  Untuned*         & 5:12        & +350\%    & & \\
				  (3 HP, 7 epochs) &                &                  &            & \\
				  \hline
				  Untuned*         & 5:15, 17, 19 & +237\% & & \\
				  (3 HP, 7 epochs) &          &               &            & \\
				  \hline
				  Tuned*           & 5:20        & -50.0\%       & &   \\
				  (3 HP, 7 epochs) &                &                  &            &   \\
				  \hline
				  Tuned***         & 5:47        & -51\%    &  & +28\% \\
				  (3 HP, 7 epochs) &                &                  &            &   \\
				  \hline
				  Tuned***         & 48:73      & +87\%   &  & +50\% \\
				  (3 HP, 7 epochs) &                &                  &            &   \\
				  \hline
				  Untuned*   & 25:5:145    & +12.8 \% & +19.5\%      & +26\%    \\   %%%% Fig. 7 cool
				  (3 HP, 7 epochs) &       &                 &                    &               \\
				  \hline
				  Half-tuned*& 40:10:120   & +50.0 \% & +19.5\%    & +25\%    \\   %%%% Fig. 8 very cool
				   (3 HP, 7 epochs)        & and 140:20:200 &                &                  &                \\
				   \hline
				   Leaky**    & 10:5:100   &  +62 \% & +40\% & +40\% \\  %%% Figure 5
				   (5 HP, 30 epochs)       &                  &               &            &            \\
           \hline
           PTB Bytes/Words & budget 20  & +57\% & +57\% & +57\% \\   %%% 22/36 
           (7 HP, 17 epochs)  & budget 30  & +0\% & +0\% & +0\% \\   %%% 
           (36 xps) & & & & \\
\hline
Tuned*           & 20:5:30     & +160\%  & +160\% & +160\%  \\
(3 HP, 4 epochs) &             &         &        &         \\
\hline
	\end{tabular}
		\caption{\label{main}Table of results for the speed-up of S-SH compared to random. See text and SM for additional xps, statistical validations and curves. The 36 xps correspond to different numbers of units. The two last rows have the same values for different speed-ups because there is only one LDS and one instance of random search (others have 3 instances of random search). Many experiments have a small number of epochs, but all experiments (including some in the text and SM) with larger number of epochs ($17$ to $45$) have speedup $\geq 0$ for LDS.}
	\end{table}

	We also checked that S-SH outperformed random on PTB bytes, PTB words, UBPTB bytes, UBPTB words, with budget 15, and with 11 epochs; S-SH won in all four cases for results averaged over 35 runs. The same happened with budget 60 (3 layers of stacked Lstm with 300 units in both cases).
	Detailed xps also reveal a better robustness for S-SH than for Sobol; and poor results for Halton (without scrambling) when applied on a problem with 7 parameters.
	Results also show that the performance still improves when the budget is over $100$, and additional tests in SM show that larger numbers of epochs (tested until 45 epochs) lead to positive results for S-SH compared to random with budget 20 to 125 or 150 (depending on testbeds); in particular for intermediate budgets (no significance for the largest or the smallest budgets).

%%%%%%%%%%% ICML END %%%%%%%%%%%%%%%%%%%%%%%%%%%%%%%%%%%%%%%%%%%%%%%%%%%%
}{}
\subsubsection{Experimental results: overview}                   % NOTINICML 
WIS is the scale of weights initialization. MGN is the maximum gradient norm for gradient clipping. LR is the initial learning rate. Each HP has a range, in which random (or quasirandom) values are drawn.                   % NOTINICML 
Xps is a short notation for xps. x3 means that 3 independent instances are used.                   % NOTINICML 
Table \ref{tuning} reports results around the degree of tuning - we see that when we have parameters sampled closer to the optimum, LDS loses its advantage.                   % NOTINICML 
Table \ref{leaky} reports results on the leaky-LSTM model; our purpose is not to advocate this model, just to check the performance of LDS sampling in this case.                    % NOTINICML 
\begin{table*}                   % NOTINICML 
\footnotesize                   % NOTINICML 
\supersmallifshort                   % NOTINICML 
	\center                   % NOTINICML 
\begin{tabular}{|c|c|c|c|c|c|c|}                   % NOTINICML 
\hline                   % NOTINICML 
	{{Experiment}} & Testbeds & Hyper- & Range & Budget & Samplers & Results \\                   % NOTINICML 
  {{name}} & & params & & & & \\                   % NOTINICML 
\hline                   % NOTINICML 
Tuned  & PTB & WIS   & $[0.02, 1]\times$ & 5 to 20 & Sobol             & 2 wins for Sobol \\                   % NOTINICML 
	parameters & words \& bytes,       & MGN     & $[0.02,1]\times$  & (16 xps)  & SH             & 2 for SH, 12 for \\  % NOTINICML 
(7 epochs) & Toy sequences & LR        & $[0.5,30]$            &             & Random & the 3 random instances. \\        % NOTINICML 
3 stacked LSTM         & C, AN, anbn& & & & (x3)& Opp-p-val = 0.167. \\                   % NOTINICML 
200 units,     & ABNA.& & & &     & Speed-up = -50\%.\\                   % NOTINICML 
no size gap,   & & & & & & \\                   % NOTINICML 
no fixed size  & & & & & & \\                   % NOTINICML 
\hline    % NOTINICML
Tuned          & Ditto & Ditto & Ditto & 20,25,30 & S-SH \& & 13 wins for S-SH \\  % NOTINICML
(ditto, except &       &       &       &          & Random  & (18 xps) \\  % NOTINICML
4 epochs)      &       &       &       &          &         & {\bf{p-val = 0.0498}}   \\  % NOTINICML
\hline                   % NOTINICML 
Untuned      & Ditto & Ditto  & $[0.02,1]\times$       & 5 to 12  & Ditto & 3 wins for Sobol,\\                   % NOTINICML 
parameters &        &           & $[0.002,100]\times$ & (8 xps) &         &   3 wins for SH \\                   % NOTINICML 
(7 epochs)   &       &           & $[0.001, 3000]$        &              &        &   2 wins for random \\                   % NOTINICML 
	(same testbeds) & & & & & & {\bf{p-val = 0.0498}} \\                   % NOTINICML 
   & & & & & & Speed-up +350\% \\                   % NOTINICML 
\hline                   % NOTINICML 
Untuned      & Ditto & Ditto  & Ditto                          & 5 to 15,   & Ditto & 5 wins for SH \\                   % NOTINICML 
parameters &        &           &                                  & 17 and 19&        & 4 wins for Sobol \\                   % NOTINICML 
(repeated)  &         &          &                                  & (13 xps)   &        & 4 wins for the 3 \\                   % NOTINICML 
	& & & & & & random {\bf{(p-val = 0.032)}}\\                   % NOTINICML 
  & & & & & & speed-up +237.5 \% \\                   % NOTINICML 
  \hline                   % NOTINICML 
Half-tuned  & Ditto & Ditto  & $[0.02,1]\times$        & 5 to 20   & Ditto &7 wins for SH \\                   % NOTINICML 
Parameters &         &         & $[0.006, 30]\times$   & (16 xps) &         &1 win for Sobol\\                   % NOTINICML 
(7 epochs)                    &        &         & $[0.1,200]$                &               &         & 8 wins for random\\                   % NOTINICML 
	(same testbeds)  & & & & & & random (p-val = 0.284, \\                   % NOTINICML 
	& & & & & & {\bf{p-val(SH)=0.01}}, \\                   % NOTINICML 
  & & & & & & Opp-p-val(Sobol)=0.227)\\                   % NOTINICML 
  & & & & & & Speed-up +50\%\\                   % NOTINICML 
\hline                   % NOTINICML 
\end{tabular}                   % NOTINICML 
\caption{\label{tuning}Impact of the degree of tuning (tuned means that the range of values is somehow hopefully narrow around known good values for our test cases) on the performance of LDS sampling.                   % NOTINICML 
The mentioned speed-up is defined in Section \ref{su} - in this Table, it corresponds to the speed-up for all LDS together compared to pure random.                   % NOTINICML 
	The small sample sizes lead to extreme and unstable estimates of speed-up;                   % NOTINICML 
	later xps provide more reasonable values. Results are essentially positive; later figures will give more details; and we will investigate in Table \ref{dependency_numtries} the disappointing results in the tuned setting.}                   % NOTINICML 
\end{table*}                   % NOTINICML 
\begin{table*}                   % NOTINICML 
\footnotesize\center                   % NOTINICML 
\supersmallifshort                   % NOTINICML 
\begin{tabular}{|c|c|c|c|c|c|}                   % NOTINICML 
\hline                   % NOTINICML 
 Testbeds & Hyperparams & Ranges \& budget & Samplers & Results \\                   % NOTINICML 
\hline                   % NOTINICML 
	Toy sequences .N, AN, anbn& LeakBias,          & $[-9,9] \times$     & Sobol & {\bf{p-val = 0.018}} \\                   % NOTINICML 
 with 26 letters and    & LeakStd,           & $ [0.01, 10]\times$& SH & Except for budget 20, \\                    % NOTINICML 
 max word size 5 or 10              &  MGN, WIS, & $[0.05,1] \times $  & Random (x3)& all wins come \\                   % NOTINICML 
	2 LSTM, 100 units, & LR                       & $[0.02,1]\times[5,100.]$ & NaiveDOE & from one of the 2\\                   % NOTINICML 
 with size gaps,  & & budget 20, & & LDS  (out of 6 methods). \\                   % NOTINICML 
	word size not fixed; & & 30, 40 \& 50. & & \\                   % NOTINICML 
 hence 6 testbeds. & & & & \\                   % NOTINICML 
\hline                   % NOTINICML 
\end{tabular}                   % NOTINICML 
	\caption{\label{leaky}Experiments on the leaky model, performed with budget 20, 30, 40, 50. For budget 20, 30 or 50, there was no significant p-val** for this budget alone; for budget 40 p-val**(Sobol)=0.062 and for budget 60 {\bf{p-val**(SH) = 0.009}}. Joining all xps,                   % NOTINICML 
	we get {\bf{p-val(LDS)=0.018.}} Figure \ref{leakyfig} will confirm the good behavior of LDS in this context, for a wide range of values of the budget.}                   % NOTINICML 
\end{table*}                   % NOTINICML 
\begin{table*}                   % NOTINICML 
\footnotesize\center                   % NOTINICML 
\supersmallifshort                   % NOTINICML 
\begin{tabular}{|c|c|c|c|c|c|}                   % NOTINICML 
\hline                   % NOTINICML 
 Testbeds & Hyperparameters & Budget & Samplers & Results \\                   % NOTINICML 
\hline                   % NOTINICML 
 PTB bytes,        & LR, & 15 & Sobol, S-SH, & nothing significant \\                   % NOTINICML 
       PTB words,        & MGN,&    & Random, NaiveDOE &   \\                   % NOTINICML 
       toy sequences     & WIS &    &  &  \\                   % NOTINICML 
       ABNA, AN, C and anbn &     & 20 & Ditto & nothing significant \\                   % NOTINICML 
       with 24, 25 or 26 &     &    &  & \\                   % NOTINICML 
	letters           &     &    &  & p-val*(Halton)=\\                   % NOTINICML 
       (i.e. 14 datasets)&     & 40 & Sobol, S-SH, Random (x3),  & p-val*(Scr-Halton)= \\                   % NOTINICML 
       max word size 7   &     &    & S-Sobol,S-Scrambled Halton,& p-val*(Sobol)=.321, \\                   % NOTINICML 
      no size gaps, no fixed size &     &    & NaiveDOE, S-Halton   &     p-val*(S-Sobol)=.114 \\                   % NOTINICML 
      C: vocab. growth 10,        & & & & Opp-p-val*(S-SH)=.367,\\                   % NOTINICML 
	depth 3                   & & & &  p-val(LDS)=0.103 \\                   % NOTINICML 
\hline                   % NOTINICML 
\end{tabular}                   % NOTINICML 
\caption{\label{bud}Experiments with budget 15, 20 \& 40, similar to the previous Tuned xp but with more datasets. Results are                   % NOTINICML 
	not very significant, though it looks like LDS performs better than random for budget 40. We will see in Fig. \ref{dependency_numtries} that                   % NOTINICML 
	over many budgets, in particular larger budgets, the difference becomes big and is actually quite significant in terms of saving                   % NOTINICML 
	up computational resources.}                   % NOTINICML 
\end{table*}                   % NOTINICML 
                   % NOTINICML 
                   % NOTINICML 
\subsubsection{Impact of the budget on LDS performance: Untuned, Leaky and Half-tuned settings}                   % NOTINICML 
Fig. \ref{untbud} presents results of the S-SH method for various budgets in the untuned setting. Results are questionable between 30 and 60, and for 65+ budget our favorite LDS method, namely S-SH, becomes clearly better, though the speed-up is moderate (a few dozens percents).                   % NOTINICML 
\begin{figure}                   % NOTINICML 
\center                   % NOTINICML 
\includegraphics[width=.8\linewidth]{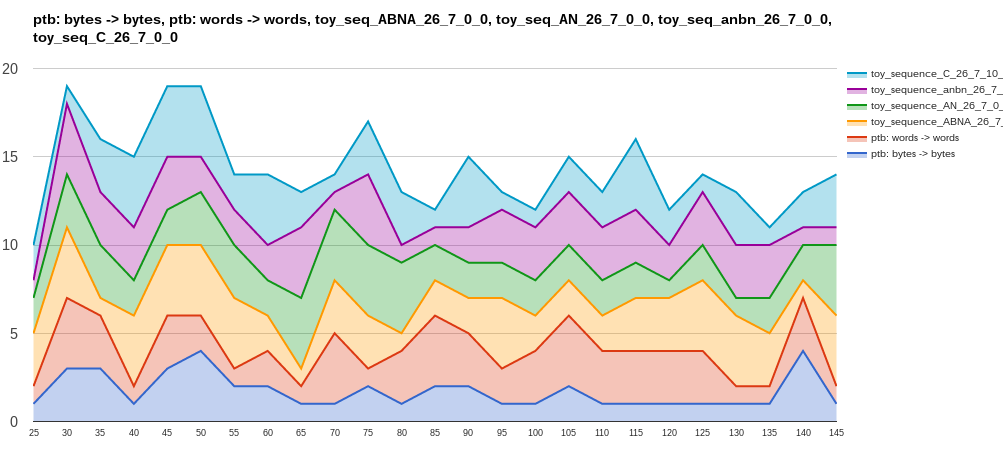}                   % NOTINICML 
\caption{\label{untbud}Results in the untuned setting, for various values of the budget. We present the rank, over 4 methods (3 instances of pure random and the S-SH method), of the S-SH method, cumulated over 6 datasets. The x-axis is the budget.                   % NOTINICML 
	Under null hypothesis the rank should be 15 on average; we see for budget sufficiently large we are almost always $< 15$, i.e. win for S-SH. The frequency of best result for S-SH leads to an estimated speed-up (as defined in Section \ref{su}) +12.8\% (average speed-up: +19.5\%; robustness-speed-up: +26\%). }                   % NOTINICML 
\end{figure}                   % NOTINICML 
                   % NOTINICML 
Then we present results in the half-tuned setting, for various values of the budget (Fig. \ref{halftuned}) (speed-up ranging between +20\% and +50\% depending on the detailed criterion);                   % NOTINICML 
and in the leaky context, in Fig. \ref{leakyfig}.  The speed-up is between +40\% and +60\% depending on the speed-up criterion. Fig. \ref{leaknaive} shows that S-SH outperforms our (expensive) homemade naive DOE.                   % NOTINICML 
\begin{figure}                   % NOTINICML 
	\center                   % NOTINICML 
	\includegraphics[width=.8\linewidth]{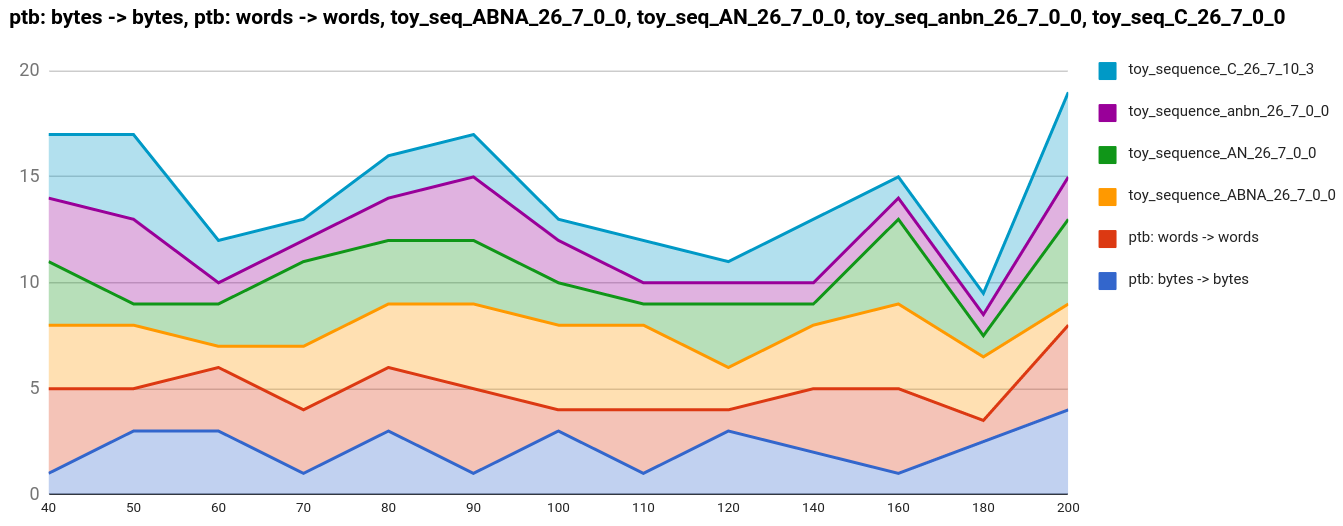}                   % NOTINICML 
	\includegraphics[width=.8\linewidth]{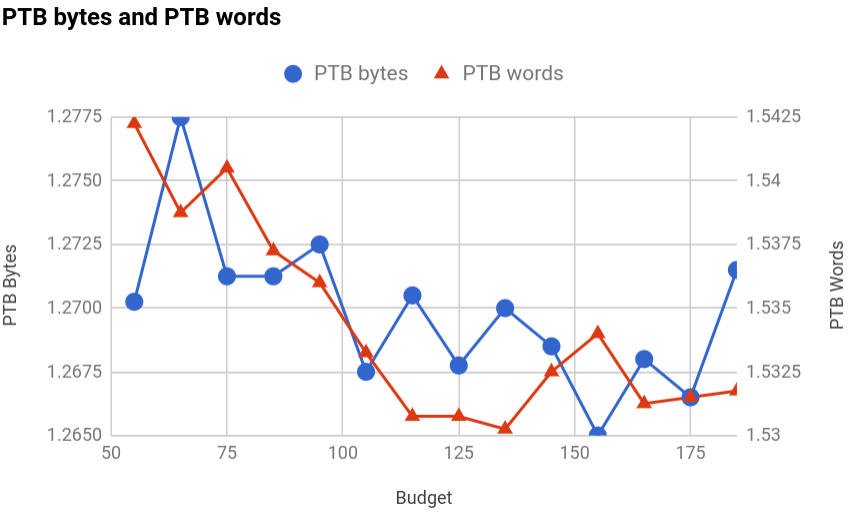}                   % NOTINICML 
	\caption{\label{halftuned}Top: Half-tuned setting, rank of S-SH among 4 methods (S-SH and 3 instances of pure random), summed over 6 datasets. Under the null hypothesis the expected rank is 15. S-SH usually dominates, though the difference is not big; the speed-up (see Section \ref{su}) corresponding to the frequency of win for S-SH is +50\% (average-speed-up: +19.5\%; robustness-speed-up: +25\%). Bottom: PTB-Bytes and PTB-Words, still in the half-tuned setting: moving averages of losses as a function of the budget for S-SH, showing that budgets $>100$ can help.}                   % NOTINICML 
\end{figure}                   % NOTINICML 
\begin{figure}\center                   % NOTINICML 
\includegraphics[width=.8\linewidth]{../leakleak.png}                   % NOTINICML 
\caption{\label{leakyfig}Experiments in the leaky context - the critical parameters are the leak parameters (see Fig. \ref{qrleak}) which are ranked 3rd and 4th, i.e. after                    % NOTINICML 
	the learning rate (1st) and the gradient norm clipping (2nd), so that this xp is in a setting in which the ordering of variables is suboptimal. The frequency of wins for S-SH compared to the 3 random instances corresponds to a speed-up +62\% as discussed in Section \ref{su} (average speed-up: +40\%; robustness speed-up: +40\%).}                   % NOTINICML 
\end{figure}                   % NOTINICML 
\begin{figure}\center                   % NOTINICML 
	\includegraphics[width=.8\linewidth]{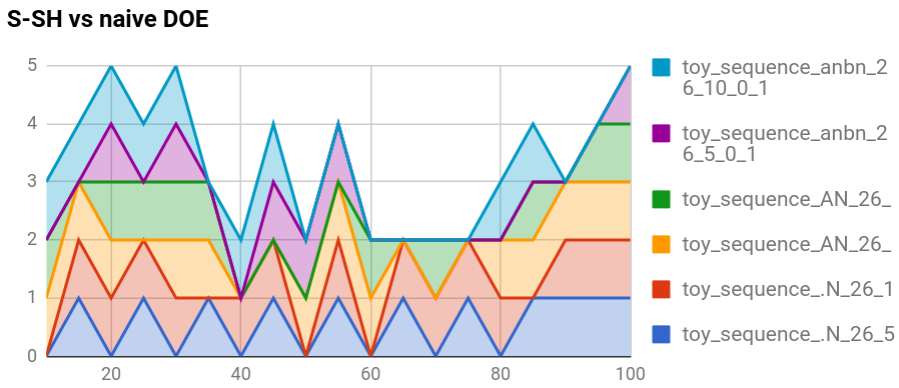}                   % NOTINICML 
	\caption{\label{leaknaive}Number of times S-SH outperforms Naive-DOE over 6 datasets, for various budgets, in the leaky context; i.e. values $>3$ means a success for S-SH compared to random. S-SH wins overall, but the p-value is 0.15 only.}                   % NOTINICML 
\end{figure}                   % NOTINICML 
Fig. \ref{sobol} compares S-SH to Sobol in the leaky and half-tuned settings respectively, as a function of the budget; we got no statistically significant difference.                   % NOTINICML 
\begin{figure}\center                   % NOTINICML 
	Untuned setting.\\                   % NOTINICML 
	\includegraphics[width=.8\linewidth]{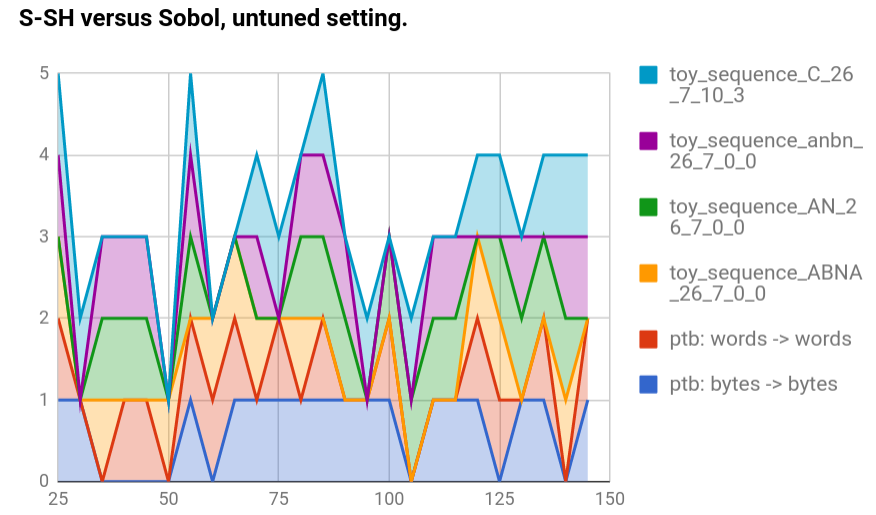}\\                   % NOTINICML 
	Leaky setting.\\                   % NOTINICML 
	\includegraphics[width=.8\linewidth]{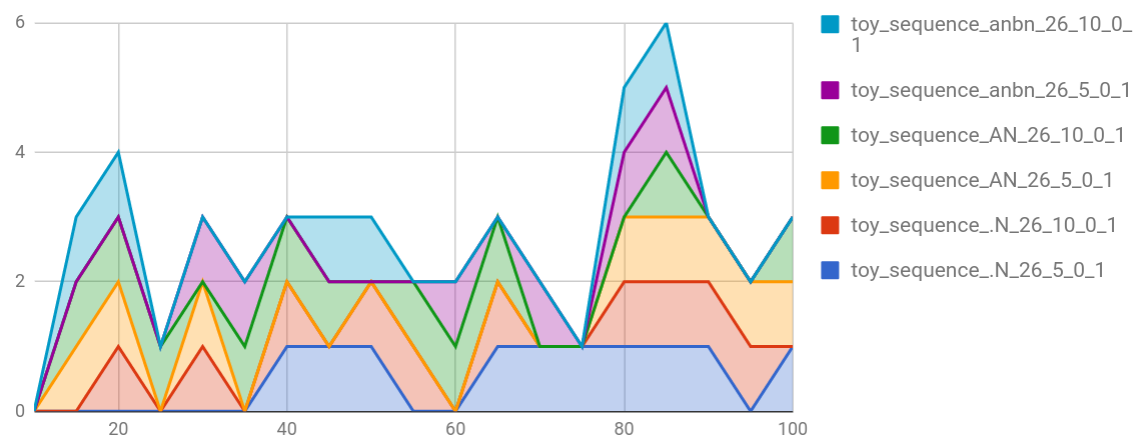}\\                   % NOTINICML 
	Half-tuned setting.\\                   % NOTINICML 
	\includegraphics[width=.8\linewidth]{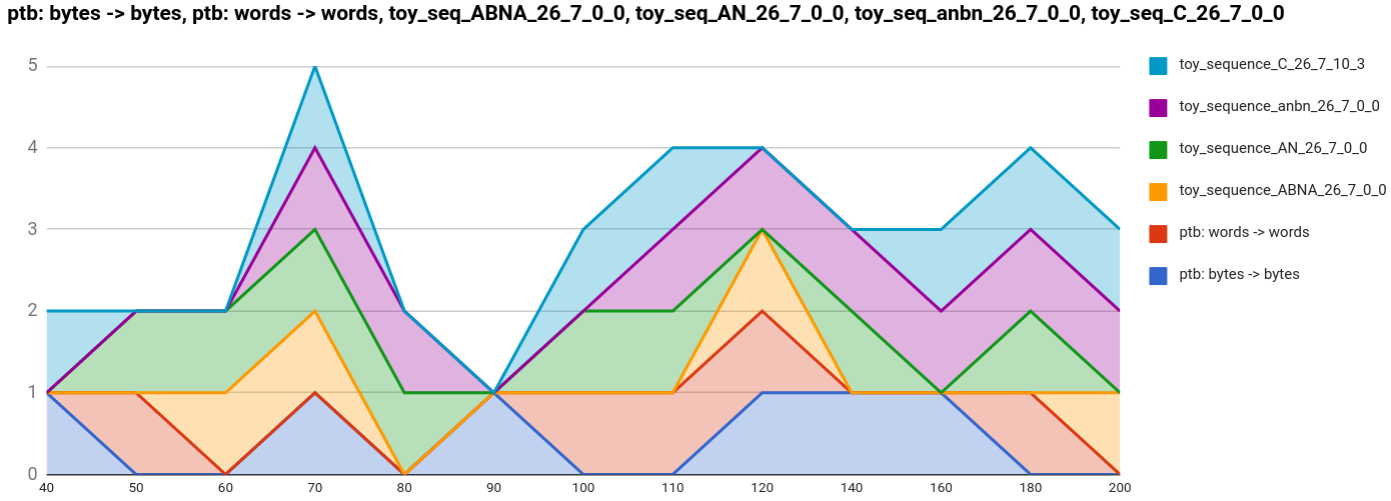}\\                   % NOTINICML 
	\caption{\label{sobol}Number of times S-SH outperforms Sobol, for various budgets, out of 6 datasets, in each of 3 settings (untuned, leaky, half-tuned).                   % NOTINICML 
	3 means equality. No clear difference overall.}                   % NOTINICML 
\end{figure}                   % NOTINICML 
We experimented the leaky setting again, but this time in the context of PTB-words, PTB-bytes, UB-PTB-words, UB-PTB-bytes;                   % NOTINICML 
results are presented in Fig. \ref{remix} (budget 15) and \ref{budget60} (budget 60), with excellent results for S-SH. Results are averaged over 35 runs.                   % NOTINICML 
\begin{figure}\center                   % NOTINICML 
	\ifthenelse{\longversion=0}{\scriptsize}{}                   % NOTINICML 
	\includegraphics[width=.8\linewidth]{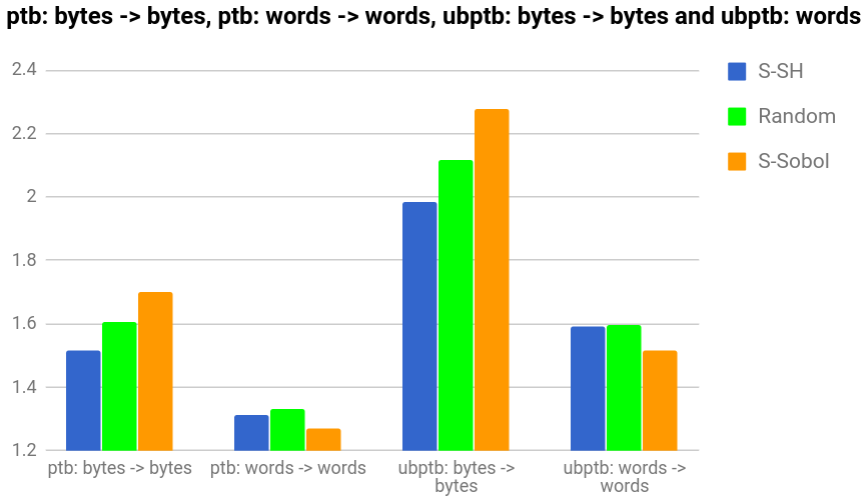}\\                   % NOTINICML 
	\scriptsize
	\begin{tabular}{c|c|c|c|c}                   % NOTINICML 
		Average & PTB-Bytes & PTB-Words & UBPTB-Bytes & UBPTB-Words \\                   % NOTINICML 
		\hline                   % NOTINICML 
		S-SH   & 1.514 $\pm$ 0.002   & 1.312$\pm$0.004  & 1.98 $\pm$ 0.006    & 1.59 $\pm$ 0.009 \\                   % NOTINICML 
		Sobol  & 1.70 $\pm$ 0.006  & 1.27$\pm$0.0028 & 2.28 $\pm$ 0.0124 & 1.51 $\pm$ 0.006 \\                   % NOTINICML 
		Random & 1.61 $\pm$ 0.003  & 1.33$\pm$0.0045 & 2.12 $\pm$ 0.0061 & 1.60 $\pm$ 0.003 \\                   % NOTINICML 
	\end{tabular}                   % NOTINICML 
	\caption{\label{remix}3 layers of stacked LSTM with 300 units, applied to 4 real-world datasets in the half-tuned setting with budget 15. S-SH outperforms                   % NOTINICML 
	   random in each case, but Sobol does not. Average of 35 runs; significance in the table (bottom). The number of epochs is moderate (11 epochs) hence the moderate performance - see Table \ref{impactofmaxepoch} for results depending on the number of epochs and Fig. \ref{ptbbyteswithbudget} for results with larger budget. p-val*(S-SH) = {\bf{0.0625}}.}                   % NOTINICML 
\end{figure}                   % NOTINICML 
\begin{figure}\center                   % NOTINICML 
	\includegraphics[width=.8\linewidth]{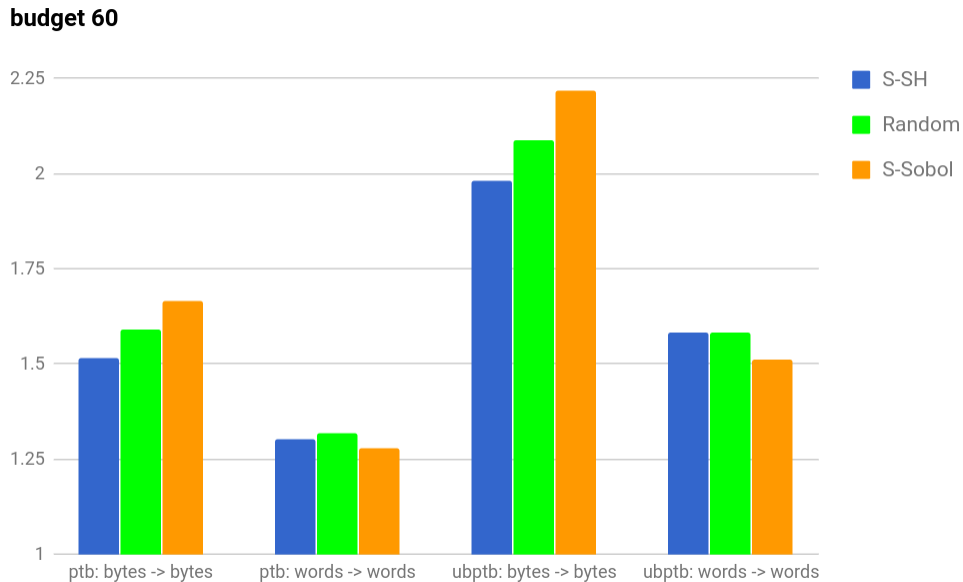}\\                   % NOTINICML 
	\caption{\label{budget60}Same xp as Fig. \ref{remix} but with budget 60. S-SH outperforms random in each case whereas Sobol does not. Average of 35 runs. p-val*(S-SH)={\bf{0.0625}}.}                   % NOTINICML 
\end{figure}                   % NOTINICML 
                   % NOTINICML 
\subsubsection{Tuned setting, impact of the budget: LDS not always beneficial for small budget}                   % NOTINICML 
We now provide more detailed experimental results for the case in which QR performed poorly,                   % NOTINICML 
namely the tuned setting, which corresponds to our platform tuned over testbeds used in                   % NOTINICML 
these xps. We tested extensively with an increasing sampling number, and report                    % NOTINICML 
the best/worst in each case; 3 independent random instances are compared to a scrambled                    % NOTINICML 
Hammersley; which means that under null assumption (the null assumption is that                    % NOTINICML 
scrambled Hammersley performs equally                    % NOTINICML 
to random) we would get Scrambled Hammersley best 25\% of runs and worst 25\% of runs;                   % NOTINICML 
in particular, we would have Scrambled Hammersley the same number of times on both sides.                    % NOTINICML 
Results are presented in Table \ref{dependency_numtries} and suggest that S-SH                    % NOTINICML 
\begin{itemize}                   % NOTINICML 
	\item is outperformed by random for low budget ($\leq 30$) in terms of frequency of best performance ({\bf{p-value 0.026}});                   % NOTINICML 
	\item but performs better than random for low budget ($\leq 30$) in terms of frequency of worst performance (p-value 0.18);                   % NOTINICML 
\end{itemize}                   % NOTINICML 
and then becomes competitive at budget circa 30 and clearly better at                   % NOTINICML 
budget circa 55; overall, S-SH:                   % NOTINICML 
\begin{itemize}                   % NOTINICML 
	\item is outperformed by random for low budget ($< 48$) in terms of frequency of best performance (p-value 0.18, speed-up $-51\%$);                   % NOTINICML 
	\item but performs better than random for low budget ($< 48$) in terms of frequency of worst performance (p-value 0.09; robustness speed-up $+28\%$);                   % NOTINICML 
	\item performs better than random for larger budget ($\geq 48$) both in terms of best performance (speed-up $+87\%$) and worst performance (robustness speed-up $+50\%$).     % NOTINICML 
\end{itemize}                   % NOTINICML 
%TODO repeat the values between budget 5 and 10 for clearly concluding that S-SH is worse than random here (not that clear for the moment, right ?)                   % NOTINICML 
\begin{table}                   % NOTINICML 
\smallifshort                   % NOTINICML 
\center                   % NOTINICML 
\begin{tabular}{|c|c|c|}                   % NOTINICML 
\hline                   % NOTINICML 
Budget & Worst method & Best method \\                   % NOTINICML 
\hline                   % NOTINICML 
\hline                   % NOTINICML 
5&	  S-SH 	 & random \\                   % NOTINICML 
6-9&	  random 	 & random \\                   % NOTINICML 
9&	  S-SH 	 & random \\                   % NOTINICML 
10&	  S-SH 	 & random \\                   % NOTINICML 
11-14 &	  random 	 & random \\                   % NOTINICML 
15&	  random 	 & S-SH \\                   % NOTINICML 
16-21&	  random 	 & random \\                   % NOTINICML 
22&	  S-SH 	 & random \\                   % NOTINICML 
23-26&	  random 	 & random \\                   % NOTINICML 
27&	  random 	 & S-SH \\                   % NOTINICML 
28-31&	  random 	 & random \\                   % NOTINICML 
32&	  random 	 & S-SH \\                   % NOTINICML 
33&	  S-SH 	 & random \\                   % NOTINICML 
34&	  random 	 & S-SH \\                   % NOTINICML 
35&	  S-SH 	 & random \\                   % NOTINICML 
36&	  random 	 & S-SH \\                   % NOTINICML 
37-40&	  random 	 & random \\                   % NOTINICML 
41&	  S-SH 	 & random \\                   % NOTINICML 
42&	  random 	 & random \\                   % NOTINICML 
43&	  random 	 & S-SH \\                   % NOTINICML 
44-45&	  random 	 & random \\                   % NOTINICML 
46&	  S-SH 	 & random \\                   % NOTINICML 
47&	  random 	 & random \\                   % NOTINICML 
\hline                   % NOTINICML 
\end{tabular}                   % NOTINICML 
\ \ \ \                    % NOTINICML 
\begin{tabular}{|c|c|c|}                   % NOTINICML 
\hline                   % NOTINICML 
Budget & Worst method & Best method \\                   % NOTINICML 
\hline                   % NOTINICML 
\hline                   % NOTINICML 
48-49&	  S-SH 	 & random \\                   % NOTINICML 
50&	  random 	 & S-SH \\                   % NOTINICML 
51&	  random 	 & random \\                   % NOTINICML 
52&	  S-SH 	 & random \\                   % NOTINICML 
53&	  random 	 & random \\                   % NOTINICML 
54&	  random 	 & S-SH \\                   % NOTINICML 
55-56&	  random 	 & random \\                   % NOTINICML 
57&	  random 	 & S-SH \\                   % NOTINICML 
58&	  random 	 & random \\                   % NOTINICML 
59-60&	  random 	 & S-SH \\                   % NOTINICML 
61-62&	  random 	 & random \\                   % NOTINICML 
63-64&	  random 	 & S-SH \\                   % NOTINICML 
65-66&	  random 	 & random \\                   % NOTINICML 
67&	  S-SH 	 & random \\                   % NOTINICML 
68-69&	  random 	 & random \\                   % NOTINICML 
70-72&	  random 	 & S-SH \\                   % NOTINICML 
73&	  random 	 & random \\                   % NOTINICML 
\hline                   % NOTINICML 
\end{tabular}                   % NOTINICML 
\caption{\label{dependency_numtries}Worst and best method for different budgets, for the Tuned setting (from previous xps, the Tuned setting is the least favorable to S-SH when the budget is small). 3 independent instances of random compete with S-SH. Under the null assumption, S-SH should appear as often on the left and on the right of this table.                   % NOTINICML 
The frequency of win on the right hand side table corresponds to a speed-up +87\%. The frequency of win on the left hand side table (budget $<$48) corresponds to a speed-up -51\%, i.e. detrimental results - but the frequency of worst result is smaller than under null assumption ``S-SH equivalent to random''.}                   % NOTINICML 
\end{table}                   % NOTINICML 
Experiments with SemiQR did not provide better results for small budget.                   % NOTINICML 
                   % NOTINICML 
%In order to quantify the progress in absolute values, and not only in terms of statistical validation, we report results on 6 toy sequences in Table \ref{r405060}, with budget 40, 50 and 60 respectively for the leak xp discussed above. In short, S-SH outperformed the 3 random instances twice (out of 6 datasets) for budget 40 (also ranking last twice), twice out of 6 datasets for budget 50 (also ranking last twice), and 5 times out of 6 for budget 60 (ranking 3rd out of 4 for the only case it did not win). Though significance is an issue, it looks like random and S-SH get similar results for budget 40 and 50 and S-SH clearly wins for budget 60.                    % NOTINICML 
We now switch to more extensive xps for quantifying the improvement beyond statistical significance.                   % NOTINICML 
                   % NOTINICML 
%\begin{figure}                   % NOTINICML 
%TODOTODO more xps in progress, see otdashboard and OTplots2                   % NOTINICML 
%	\caption{\label{r405060}TODO 70 and 80 are coming}                   % NOTINICML 
%\end{figure}                   % NOTINICML 
                   % NOTINICML 
\subsubsection{Tuned setting, application to PTB: quantifying the improvement in a difficult setting}\label{epoch45}                   % NOTINICML 
S-SH was disappointing in the tuned setting when applied to PTB-words (though the difference was moderate and in terms of robustness-speedup S-SH was still beneficial); we here experiment it on a larger scale.                   % NOTINICML 
Figures \ref{ptbbyteswithbudget} and \ref{ptbwordswithbudget} present experimental results for the tuned setting (i.e. the most difficult for LDS according to xps above) for budget 20,25,40,45,50,\dots,95,100,110,120,\dots,170,180. We see that S-SH outperforms random for budgets larger than above.                   % NOTINICML 
\begin{figure}                   % NOTINICML 
	\center                   % NOTINICML 
	\includegraphics[width=.8\linewidth]{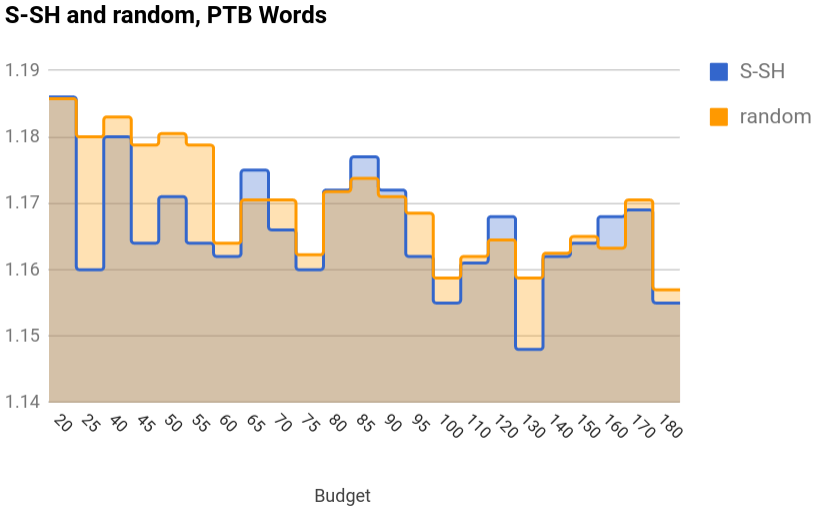}                   % NOTINICML 
	\includegraphics[width=.8\linewidth]{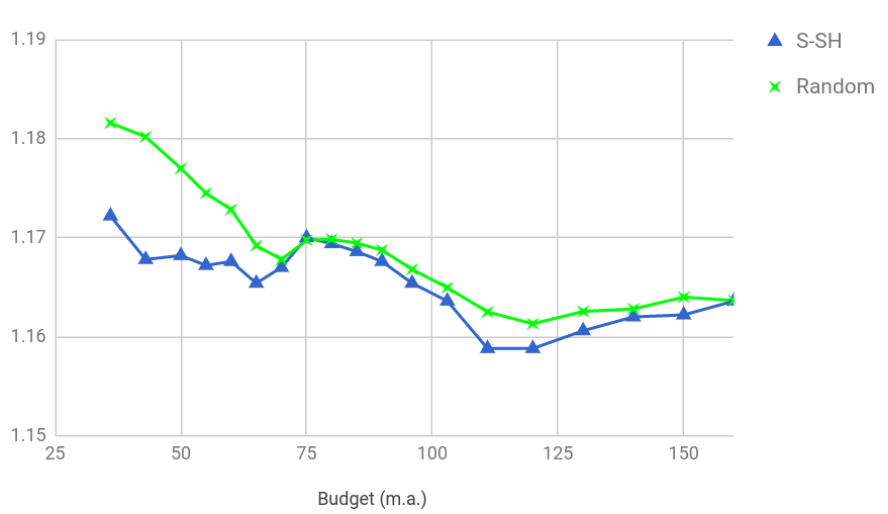}                   % NOTINICML 
	\caption{\label{ptbbyteswithbudget}PTB-words, Tuned setting (with moving average, bottom): S-SH clearly outperforms pure random (averaged over two runs) for budgets between 40 and 85. For larger budgets or smaller budgets the difference looks like noise. We also see that performance seemingly still improves as a function of the budget with budget $>80$ (independently of the comparison LDS/random). These xps have been performed with 45 epochs.}                   % NOTINICML 
\end{figure}                   % NOTINICML 
                   % NOTINICML 
\begin{figure}                   % NOTINICML 
	\center                   % NOTINICML 
	\includegraphics[width=.8\linewidth]{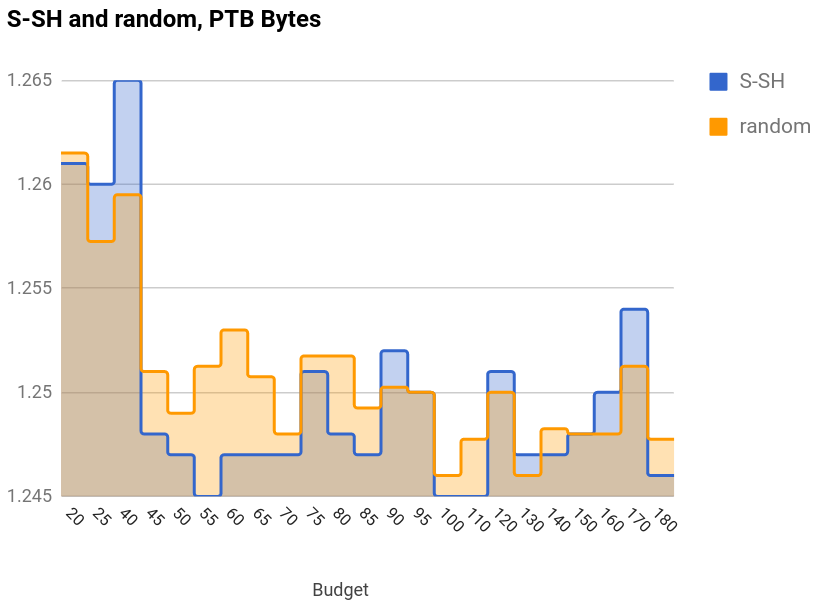}                   % NOTINICML 
	\includegraphics[width=.8\linewidth]{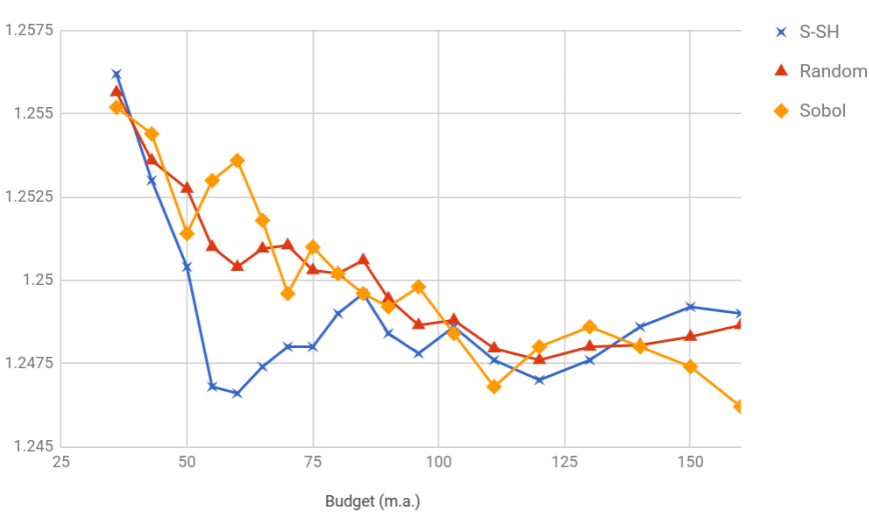}                   % NOTINICML 
	\caption{\label{ptbwordswithbudget}PTB-bytes, Tuned setting (with moving average, bottom): S-SH seemingly outperforms random (averaged over 2 runs) for intermediate budgets. For larger budgets or smaller budgets the difference looks like noise. We also see that performance seemingly still improves as a function of the budget (independently of the comparison LDS/random) with budget $>100$. These xps have been performed with 45 epochs.}                   % NOTINICML 
\end{figure}                   % NOTINICML 
                   % NOTINICML 
\subsubsection{Validating scrambling/Hammersley on PTB: not all LDS are equivalent}\label{xp7hp}                   % NOTINICML 
                   % NOTINICML 
Fig. \ref{scr} compares pure random, Halton, and scrambled Halton on PTB-Bytes                   % NOTINICML 
and PTB-Words. The setting is as follows: 7 HP (dropout keep probability in $[0.2,1]$,                    % NOTINICML 
learning rate in $[0.05,300]$, gradient clipping norm in $[0.002,1]$, Adam's epsilon parameter in $[0.001,2]$,                    % NOTINICML 
weight initialization scale in $[0.002,10]$, epoch index for starting the exponential decay of                    % NOTINICML 
learning rate in $[5,15]$, learning rate decay in $[0.1,1]$);                   % NOTINICML 
17 training epochs, 2 stacked LSTM; we perform xps for a number of units ranging from 12 to 29.                   % NOTINICML 
The budget for the randomly drawn HPs is 20.                   % NOTINICML 
Overall, there are 36 comparisons (18 on PTB-Bytes, corresponding to 18 different numbers of units, and 18 on PTB-Words);                    % NOTINICML 
\begin{itemize}                   % NOTINICML 
	\item Scrambled-Hammersley outperforms Halton 25 times (p-value {\bf{0.036}});                   % NOTINICML 
	\item Scrambled-Hammersley outperforms random 22 times (p-value 0.12);                   % NOTINICML 
\item Halton outperforms random 19 times (p-value 0.43).                   % NOTINICML 
\end{itemize}                   % NOTINICML 
The xp was reproduced a second time, with 30 random tries for the HPs. Results are presented in Fig. \ref{scrambling2} - no statistically significant improvement.                   % NOTINICML 
                   % NOTINICML 
\begin{figure}                   % NOTINICML 
\center                   % NOTINICML 
\includegraphics[width=.8\linewidth]{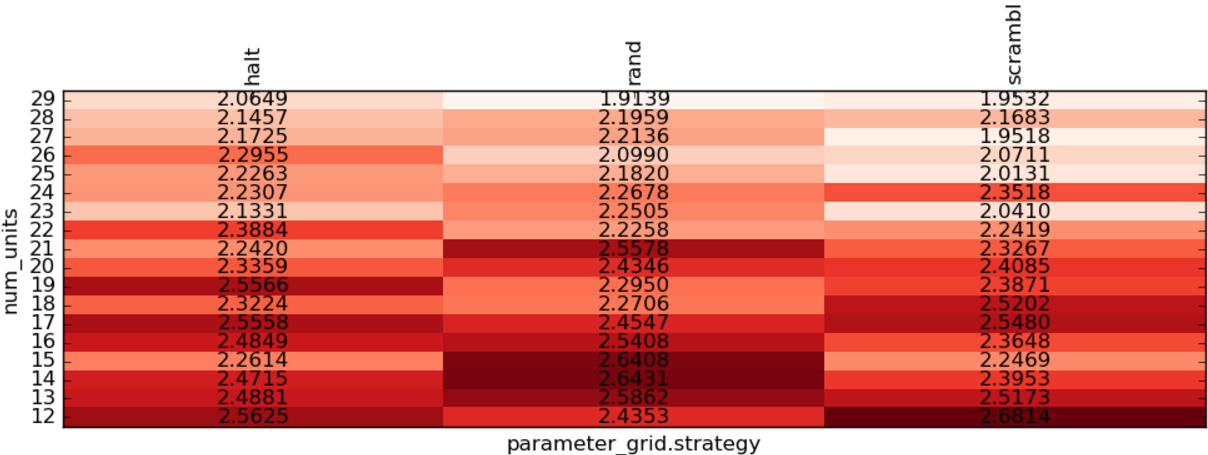}                   % NOTINICML 
\includegraphics[width=.8\linewidth]{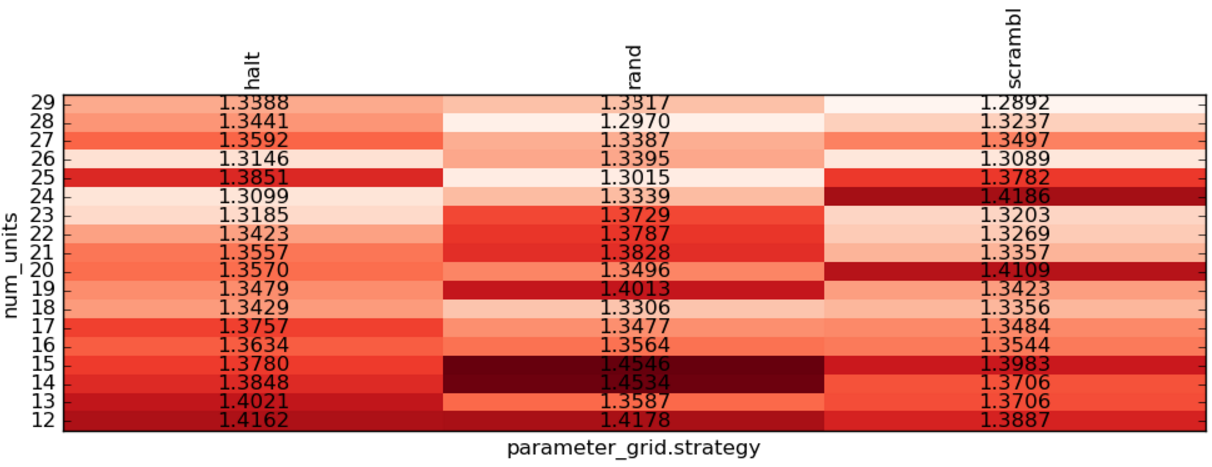}                   % NOTINICML 
	\caption{\label{scr}Comparing a sophisticated Halton to a naive Halton and to random with 17 learning epochs. Halton refers to the original Halton sequence. Scramb. refers to Hammersley with scrambling - which has the best known discrepancy bounds (more precisely the best proved bounds are obtained by Atanassov's scrambling; for the random scrambling we use, as previously mentioned, it is conjectured that the performance is the same). Top: PTB-Bytes. Bottom: PTB-Words. Scrambled-Hammersley outperforms the simple Halton and pure random (see text).}                   % NOTINICML 
\end{figure}                   % NOTINICML 
\begin{figure}                   % NOTINICML 
\center                   % NOTINICML 
\includegraphics[width=.8\linewidth]{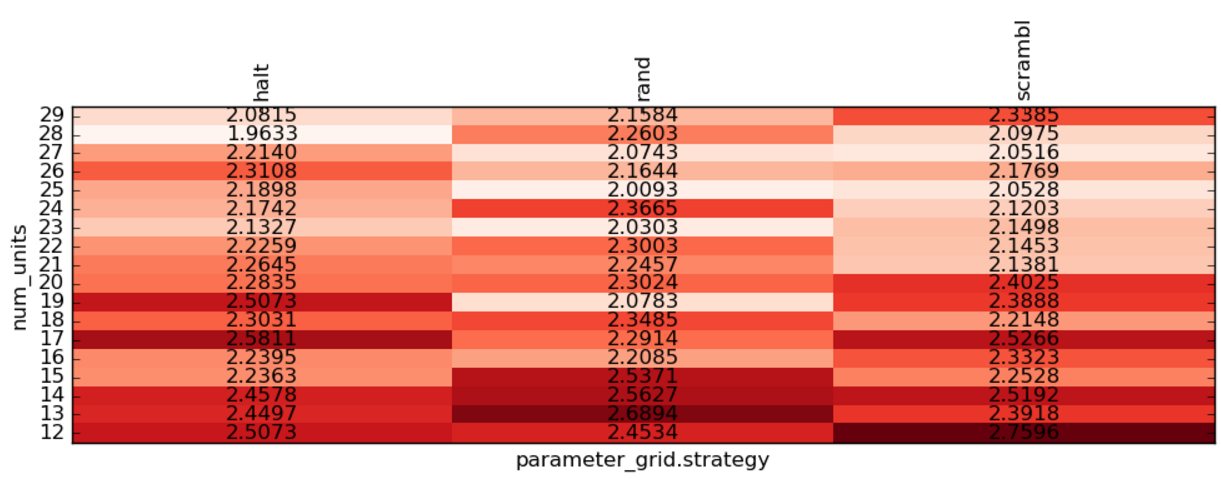}                   % NOTINICML 
\includegraphics[width=.8\linewidth]{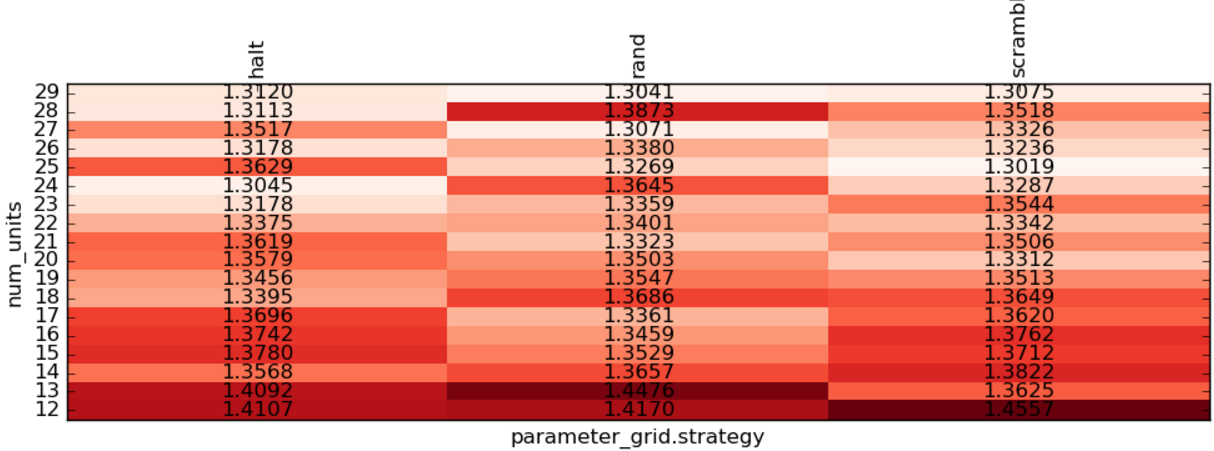}                   % NOTINICML 
\caption{\label{scrambling2}Same as Fig. \ref{scr} but with budget 30 instead of 20, still 17 learning epochs. Top: PTB-Bytes. Bottom: PTB-Words.                    % NOTINICML 
No statistically significant difference neither for bytes (9 wins for 18 test cases, 9/18 and 10/18 for S-SH vs random,                   % NOTINICML 
	for Halton vs rand, and for S-SH vs Halton respectively) or words (9/18, 10/18 and 9/18 respectively).}                   % NOTINICML 
\end{figure}                   % NOTINICML 
                   % NOTINICML 
\subsubsection{Impact of the number of epochs and of a small budget}                   % NOTINICML 
                   % NOTINICML 
We consider the untuned setting, on the same 6 problems. We have a number of epochs ranging 
from 7 to 36, and we consider moving averages of the ranks over the 6 datasets and 4 successive numbers of epochs.                   % NOTINICML 
Fig. \ref{impactofmaxepoch} presents the impact of the number of epochs; S-SH performs best overall.                   % NOTINICML 
                   % NOTINICML 
\begin{figure}                   % NOTINICML 
\center                   % NOTINICML 
\includegraphics[width=.7\linewidth]{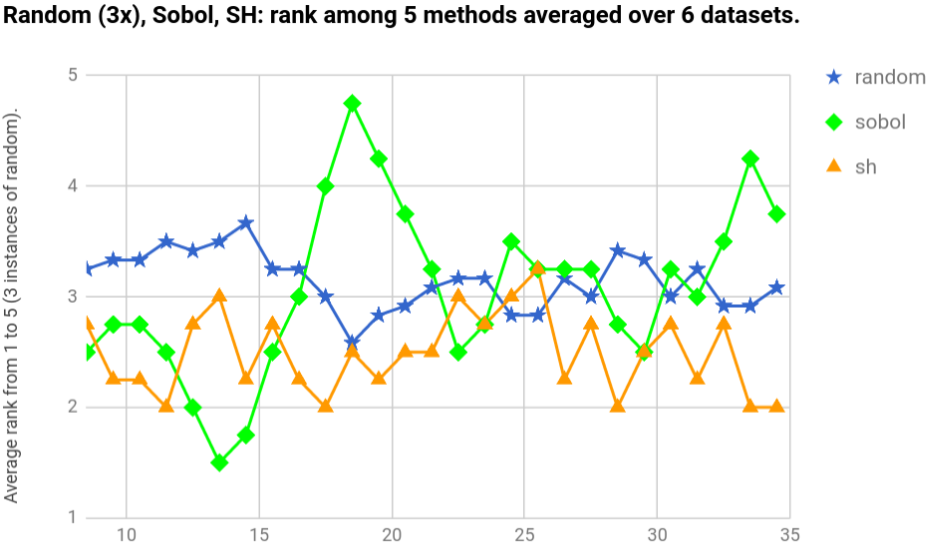}                   % NOTINICML 
\caption{\label{impactofmaxepoch}Untuned setting; rank of each method among 5 methods (3 instances of random, plus Sobol and Scrambled-Hammersley), averaged over 6 datasets and 4 successive numbers of epochs (i.e. each point is the average of 24 results). This figure corresponds to a budget of 20 vectors of HPs; Scrambled Hammersley outperforms random; Sobol did not provide convincing results. We also tested a budget 10 and results were looking like random noise.}                   % NOTINICML 
\end{figure}                   % NOTINICML 
%ptb: bytes -> bytes	ptb: words -> words	toy_sequence_ABNA_26_7_0_0	toy_sequence_AN_26_7_0_0	toy_sequence_anbn_26_7_0_0	toy_sequence_C_26_7_10_3                   % NOTINICML 
