# Supplementary material for: Critical Hyper-Parameters: No Random, No Cry
Source: arXiv:1706.03200 source file (2017-06-10)
Supplement: Supplementary file 2 [file appendix_toy.tex]

\section{Learning-free tests of LDS and other sampling methods}\label{appendix:toy}
Deep learning can be quite expensive; therefore we first propose preliminary
fast xps, used as unit tests and visual validation tools.
Real world xps are presented in Section \ref{endtoend}.

\subsection{Optimization-free tests on LDS}
Experimenting in the context of optimization is highly time consuming, so
we first present simple tools that we use as unit tests for validating our
implementations.

\paragraph{Probability of finding a set.}
We performed xps similar to those in \cite{BergtraBengio}, with
different sets:
\begin{itemize}
\item The set of admissible points is defined by $10x + y + z\leq 129$, where $x\in [10,20], y\in [0,100], z\in \{10,11,12,\dots,20\}$.
\item The discrete feature $z$ is obtained by discretization of $[10,20]$.
\item 7 pointless features (no impact on the validity of points) are added, so we have 10 variables.
\end{itemize}

We show the difference between random and quasirandom as follows:
\begin{itemize}
	\item With quasirandom points, 30 samples of 50 000 points are drawn. The runs
	are randomized by discarding a random initial segment of points. 
  Each of these 30 runs
	successfully finds 500 points in the feasible set.
	\item With random points, 10 groups of 10 samples of 50 000 points are
  randomly drawn; each of these
	groups contains at least one failure (and often more).
\end{itemize}
This is integrated as a unit test and validates a robustness property, compared
to random sampling: while quasirandom succeeds 30 times in a row, groups of 10
are very likely to fail for random.
For rectangles with axes parallel to the basis, discrepancy ensures a stable
sampling - these xps show that it works as well on this not-axis-parallel setup. 

\paragraph{Validating scrambling by correlations.}
We consider the 5000 first points for Halton, compared to the 5000 first points
for scrambled Halton. Then, we extracted the vector of the 55 correlations
(absolute values) between coordinates 40 to 50 (each pair of coordinates is
considered, hence 11x10/5 correlations).

We got an average absolute value of correlation 0.061 for Halton points; and
0.0096 for Scrambled Halton points (mean minus 2 standard deviations = 0.039 for
Halton, mean plus 2 standard deviations = 0.011 for scrambled Halton). This is
now included as a unit test for validating high dimensional quasirandom
sequences. This confirms the intuition behind Fig. \ref{scrfig}.

\subsection{Validating sampling by best value in optimization of toy
	    deterministic functions}\label{tsamp}
We loop over dimensions 2, 4, 8, and 16; we check three objective functions,
namely the sphere ($f(x)=||x-x^*||$), illcond 
($f(x) = \sum_{i=1}^d (d-i)^3(x_i-x^*_i)^2$), reverseIllcond 
($f(x)= \sum_{i=1}^d (1+i)^3(x_i-x^*_i)^2$). The budget is $n=37$ in all cases.
We used antithetic variables, thanks to mirroring w.r.t the 3 first axes (hence
8 symmetries). Each method is tested with and without this 3D mirroring. 3D mirroring
deals conveniently with multiples of 8; additional points are generated in a pure
random manner. $x^*$ is randomly drawn uniformly in the domain. Each of these 12
xps is reproduced 1221 times.

Compared methods are one-shot optimization algorithms based on the following samplings:
 Random;
 Naive DOE (DOE stands for Design of Experiments);
 LHS;
 Sobol;
 Hammersley;
 Halton;
 Scrambled Hammersley;
 SemiQR (in which half points are generated with Scrambled Hammersley, and half points by simple pure random).

Naive DOE works as follows:
\begin{itemize}
\item Randomly draw 11 samplings $S_1,\dots,S_{11}$, $n$ points each, in a
      purely randomized manner.
\item Compute their dispersion 
      $disp_i = \max_{x\in [0,1]^d} \min_{s\in S_i} ||x-s||$.
\item Return the sampling $S_i$ such that $disp_i$ is minimum.
\end{itemize}
A large number (rather than 11) leads to grid-like sampling, which perform poorly; basically this naive DOE is a kind of random search
except that we reject samplings with big holes.

Results are as follows:
\begin{itemize}
	\item In each of these 12 cases (4 different dimensions $\times$ 3 different test functions), on average over the 1221 runs, Sobol and
      Scrambled-Hammersley performed better than Random (this is now part of the unit tests). 
      This validates, on these artificial problems,
      both Sobol and Scrambled-Hammersley, in terms of one-shot optimization and 
      face to random search, with {\bf{p-value 0.0002}}.
\item Unsurprisingly, for illcond, Halton and Hammersley outperform random, whereas
      it is the opposite for reverseIllcond at least in dimension 8 and 16,
      i.e. it matters to have the most important variables first (see detailed
      results in appendix). Scrambled versions (both Halton and Hammersley) resist
      much better and still outperform random - this validates scrambling.
\item Scrambled Hammersley performs best 6 times, scrambled Halton and
      Hammersley 2 times each, Sobol and Halton once each;  none of the 3d
      mirrored tools ever performed best. This invalidates mirroring, and confirm the
      good behavior of scrambled Hammersley.
\end{itemize}
Detailed results are presented in Section \ref{detailedtoyxps}.

\subsection{Deceptive functions: the practice of advanced samplings failures}

\paragraph{A deceptive function for Sobol.}
We define the following AntiSobol function: $f_{antisobol}(x) =( (x_1 -x^*_1)+(x_2-x^*_2))^2$. The formula is the same in arbitrary dimension, so that coordinates of index $>2$ are ignored; this function is
not defined in dimension 1. We use the same experimental setup as in Section \ref{tsamp}, i.e. 1221 runs for each considered dimension, and an optimum $x^*$ uniformly drawn in $[0,1]^d$.
We use the same 8 methods. We reproduce this xp 30 times (each time we average 1221 runs), for each dimension in 2,3,4,\dots,9. Out of these $30\times 8$ xps, Sobol was never ranked first, it was ranked second once, and for each dimension it was ranked last at least 12 times out of 30. Random performed much better in all dimensions.
On this function, on the other hand, Scrambled Hammersley was ranked first 
13, 17, 10, 13, 14, 12, 7, 16 times out of 30 in dimension 2,3,4,5,6,7,8 and 9 respectively, among these 8 samplers.
Detailed results are presented in Table \ref{antisobol}.

\paragraph{A deceptive function for randomly shifted Scrambled Hammersley.}
We use $f_{antish}=(\sum_{1\leq i \leq d} x_i-x^*_i)^2$ as a deceptive (diagonal) function for S-SH in dimension $d$. In dimension 2 to 9, results were in favor of random (compared to S-SH), still with budget=37; and the gap is wider in dimension 12 to 18. However, the gap is far less clear than for the Sobol-deceptive function - scrambled Hammersley looks like a robust alternative in the sense that we did not find ``very'' deceptive functions for S-SH.
Detailed results are presented in Table \ref{antish}.

\section{Artificial objective functions: detailed results}\label{detailedtoyxps}
This section presents detailed results of LDS, random search and other sampling methods for one-shot optimization.

\subsection{Artificial xps on quasirandom, with most important variables first for illcond}                                                             % NOTINICML
We here consider the sphere objective function (for which all variables are equally important) and the illcond objective function (for which the first variables are the most important).                                                             % NOTINICML
Results are presented in Table \ref{illcondcool}. For the sphere the best results are always obtained by a scrambled method; for illcond (for which only the few first variables matter) the best results                                                             % NOTINICML
are always obtained by a LDS and the different LDS perform equally.                                                             % NOTINICML
                                                             % NOTINICML
\begin{table*}\center                                                             % NOTINICML
{\scriptsize{                                                             % NOTINICML
\begin{tabular}{|c|c|}                                                             % NOTINICML
	\hline                                                             % NOTINICML
\multicolumn{2}{c}{Ranking in dimension 2, sphere}\\                                                             % NOTINICML
	\hline                                                             % NOTINICML
S-SH & 0.0054$\pm$0.0001\\                                                             % NOTINICML
Hammersley & 0.0057$\pm$0.0001\\                                                             % NOTINICML
Halton & 0.0061$\pm$0.0001\\                                                             % NOTINICML
scr-Halton & 0.0062$\pm$0.0001\\                                                             % NOTINICML
scr-Halton3dmirror & 0.0063$\pm$0.0001\\                                                             % NOTINICML
sobol & 0.0074$\pm$0.0001\\                                                             % NOTINICML
Hammersley3dmirror & 0.0077$\pm$0.0001\\                                                             % NOTINICML
naivedoe3dmirror & 0.0077$\pm$0.0001\\                                                             % NOTINICML
naivedoe & 0.0080$\pm$0.0001\\                                                             % NOTINICML
S-SH3dmirror & 0.0080$\pm$0.0002\\                                                             % NOTINICML
random3dmirror & 0.0082$\pm$0.0002\\                                                             % NOTINICML
Halton3dmirror & 0.0086$\pm$0.0002\\                                                             % NOTINICML
lhs & 0.0087$\pm$0.0002\\                                                             % NOTINICML
sobol3dmirror & 0.0090$\pm$0.0002\\                                                             % NOTINICML
random & 0.0092$\pm$0.0002\\                                                             % NOTINICML
lhs3dmirror & 0.0101$\pm$0.0003\\                                                             % NOTINICML
	\hline                                                             % NOTINICML
\multicolumn{2}{c}{Ranking in dimension 2, illcond}\\                                                             % NOTINICML
	\hline                                                             % NOTINICML
Hammersley & 0.0155$\pm$0.0003\\                                                             % NOTINICML
S-SH & 0.0155$\pm$0.0003\\                                                             % NOTINICML
scr-Halton & 0.0170$\pm$0.0004\\                                                             % NOTINICML
Halton & 0.0172$\pm$0.0004\\                                                             % NOTINICML
scr-Halton3dmirror & 0.0207$\pm$0.0005\\                                                             % NOTINICML
lhs3dmirror & 0.0229$\pm$0.0007\\                                                             % NOTINICML
lhs & 0.0243$\pm$0.0007\\                                                             % NOTINICML
Hammersley3dmirror & 0.0244$\pm$0.0007\\                                                             % NOTINICML
Halton3dmirror & 0.0247$\pm$0.0005\\                                                             % NOTINICML
sobol & 0.0257$\pm$0.0007\\                                                             % NOTINICML
S-SH3dmirror & 0.0259$\pm$0.0008\\                                                             % NOTINICML
sobol3dmirror & 0.0261$\pm$0.0007\\                                                             % NOTINICML
random & 0.0261$\pm$0.0008\\                                                             % NOTINICML
naivedoe3dmirror & 0.0263$\pm$0.0008\\                                                             % NOTINICML
naivedoe & 0.0275$\pm$0.0007\\                                                             % NOTINICML
random3dmirror & 0.0345$\pm$0.0011\\                                                             % NOTINICML
	\hline                                                             % NOTINICML
\multicolumn{2}{c}{Ranking in dimension 4, sphere}\\                                                             % NOTINICML
	\hline                                                             % NOTINICML
S-SH & 0.0716$\pm$0.0011\\                                                             % NOTINICML
Hammersley & 0.0728$\pm$0.0011\\                                                             % NOTINICML
Halton & 0.0755$\pm$0.0013\\                                                             % NOTINICML
S-SH3dmirror & 0.0769$\pm$0.0013\\                                                             % NOTINICML
naivedoe & 0.0773$\pm$0.0013\\                                                             % NOTINICML
scr-Halton & 0.0779$\pm$0.0013\\                                                             % NOTINICML
sobol & 0.0783$\pm$0.0013\\                                                             % NOTINICML
lhs & 0.0815$\pm$0.0013\\                                                             % NOTINICML
Hammersley3dmirror & 0.0842$\pm$0.0015\\                                                             % NOTINICML
random & 0.0873$\pm$0.0017\\                                                             % NOTINICML
lhs3dmirror & 0.0906$\pm$0.0014\\                                                             % NOTINICML
naivedoe3dmirror & 0.0942$\pm$0.0018\\                                                             % NOTINICML
sobol3dmirror & 0.0974$\pm$0.0016\\                                                             % NOTINICML
Halton3dmirror & 0.1019$\pm$0.0019\\                                                             % NOTINICML
scr-Halton3dmirror & 0.1034$\pm$0.0021\\                                                             % NOTINICML
random3dmirror & 0.1311$\pm$0.0020\\                                                             % NOTINICML
	\hline                                                             % NOTINICML
\multicolumn{2}{c}{Ranking in dimension 4, illcond}\\                                                             % NOTINICML
	\hline                                                             % NOTINICML
S-SH & 0.8254$\pm$0.0125\\                                                             % NOTINICML
Hammersley & 0.8475$\pm$0.0127\\                                                             % NOTINICML
sobol & 0.8791$\pm$0.0142\\                                                             % NOTINICML
scr-Halton & 0.9021$\pm$0.0157\\                                                             % NOTINICML
Halton & 0.9154$\pm$0.0161\\                                                             % NOTINICML
S-SH3dmirror & 0.9690$\pm$0.0150\\                                                             % NOTINICML
Hammersley3dmirror & 0.9949$\pm$0.0158\\                                                             % NOTINICML
naivedoe & 1.0159$\pm$0.0197\\                                                             % NOTINICML
random3dmirror & 1.0467$\pm$0.0225\\                                                             % NOTINICML
Halton3dmirror & 1.0720$\pm$0.0225\\                                                             % NOTINICML
lhs & 1.0903$\pm$0.0206\\                                                             % NOTINICML
scr-Halton3dmirror & 1.0921$\pm$0.0240\\                                                             % NOTINICML
sobol3dmirror & 1.0954$\pm$0.0229\\                                                             % NOTINICML
random & 1.1211$\pm$0.0210\\                                                             % NOTINICML
lhs3dmirror & 1.1531$\pm$0.0217\\                                                             % NOTINICML
naivedoe3dmirror & 1.8661$\pm$0.0415\\                                                             % NOTINICML
	\hline                                                             % NOTINICML
  \end{tabular}                                                             % NOTINICML
\begin{tabular}{|c|c|}                                                             % NOTINICML
	\hline                                                             % NOTINICML
\multicolumn{2}{c}{Ranking in dimension 8, sphere}\\                                                             % NOTINICML
	\hline                                                             % NOTINICML
scr-Halton & 0.3744$\pm$0.0040\\                                                             % NOTINICML
Halton & 0.3785$\pm$0.0039\\                                                             % NOTINICML
Hammersley & 0.3816$\pm$0.0039\\                                                             % NOTINICML
sobol & 0.3853$\pm$0.0042\\                                                             % NOTINICML
S-SH & 0.3867$\pm$0.0039\\                                                             % NOTINICML
lhs & 0.3885$\pm$0.0042\\                                                             % NOTINICML
naivedoe & 0.3995$\pm$0.0045\\                                                             % NOTINICML
random & 0.4039$\pm$0.0043\\                                                             % NOTINICML
scr-Halton3dmirror & 0.4577$\pm$0.0056\\                                                             % NOTINICML
naivedoe3dmirror & 0.4723$\pm$0.0053\\                                                             % NOTINICML
lhs3dmirror & 0.4764$\pm$0.0055\\                                                             % NOTINICML
S-SH3dmirror & 0.4780$\pm$0.0060\\                                                             % NOTINICML
sobol3dmirror & 0.4859$\pm$0.0055\\                                                             % NOTINICML
random3dmirror & 0.5038$\pm$0.0055\\                                                             % NOTINICML
Hammersley3dmirror & 0.5434$\pm$0.0068\\                                                             % NOTINICML
Halton3dmirror & 0.6133$\pm$0.0076\\                                                             % NOTINICML
	\hline                                                             % NOTINICML
\multicolumn{2}{c}{Ranking in dimension 8, illcond}\\                                                             % NOTINICML
	\hline                                                             % NOTINICML
S-SH & 31.4944$\pm$0.3865\\                                                             % NOTINICML
sobol & 32.1118$\pm$0.3980\\                                                             % NOTINICML
Hammersley & 32.2906$\pm$0.3838\\                                                             % NOTINICML
Halton & 32.6409$\pm$0.3992\\                                                             % NOTINICML
scr-Halton & 32.7235$\pm$0.4049\\                                                             % NOTINICML
random & 33.5384$\pm$0.4245\\                                                             % NOTINICML
S-SH3dmirror & 33.9388$\pm$0.4340\\                                                             % NOTINICML
lhs & 34.6569$\pm$0.4283\\                                                             % NOTINICML
Hammersley3dmirror & 34.9856$\pm$0.4536\\                                                             % NOTINICML
naivedoe & 35.3151$\pm$0.4595\\                                                             % NOTINICML
scr-Halton3dmirror & 36.5532$\pm$0.4958\\                                                             % NOTINICML
Halton3dmirror & 37.8466$\pm$0.5019\\                                                             % NOTINICML
sobol3dmirror & 38.7017$\pm$0.5379\\                                                             % NOTINICML
random3dmirror & 39.1370$\pm$0.5331\\                                                             % NOTINICML
naivedoe3dmirror & 39.5667$\pm$0.5523\\                                                             % NOTINICML
lhs3dmirror & 41.4147$\pm$0.5170\\                                                             % NOTINICML
	\hline                                                             % NOTINICML
\multicolumn{2}{c}{Ranking in dimension 16, sphere}\\                                                             % NOTINICML
	\hline                                                             % NOTINICML
scr-Halton & 1.2184$\pm$0.0082\\                                                             % NOTINICML
Halton & 1.2191$\pm$0.0085\\                                                             % NOTINICML
Hammersley & 1.2246$\pm$0.0085\\                                                             % NOTINICML
sobol & 1.2278$\pm$0.0081\\                                                             % NOTINICML
lhs & 1.2415$\pm$0.0080\\                                                             % NOTINICML
S-SH & 1.2427$\pm$0.0082\\                                                             % NOTINICML
random & 1.2622$\pm$0.0085\\                                                             % NOTINICML
naivedoe & 1.2679$\pm$0.0087\\                                                             % NOTINICML
S-SH3dmirror & 1.3816$\pm$0.0102\\                                                             % NOTINICML
naivedoe3dmirror & 1.3956$\pm$0.0105\\                                                             % NOTINICML
scr-Halton3dmirror & 1.4006$\pm$0.0101\\                                                             % NOTINICML
lhs3dmirror & 1.4316$\pm$0.0099\\                                                             % NOTINICML
random3dmirror & 1.4637$\pm$0.0112\\                                                             % NOTINICML
sobol3dmirror & 1.4808$\pm$0.0104\\                                                             % NOTINICML
Hammersley3dmirror & 1.6063$\pm$0.0117\\                                                             % NOTINICML
Halton3dmirror & 1.7789$\pm$0.0132\\                                                             % NOTINICML
	\hline                                                             % NOTINICML
\multicolumn{2}{c}{Ranking in dimension 16, illcond}\\                                                             % NOTINICML
	\hline                                                             % NOTINICML
Halton & 902.1823$\pm$8.2047\\                                                             % NOTINICML
scr-Halton & 902.4184$\pm$7.7450\\                                                             % NOTINICML
Hammersley & 906.3696$\pm$7.9888\\                                                             % NOTINICML
sobol & 906.6517$\pm$7.9694\\                                                             % NOTINICML
S-SH & 911.5179$\pm$7.8684\\                                                             % NOTINICML
naivedoe & 923.0551$\pm$8.6561\\                                                             % NOTINICML
lhs & 943.5814$\pm$8.7329\\                                                             % NOTINICML
scr-Halton3dmirror & 959.4747$\pm$9.9572\\                                                             % NOTINICML
random & 961.8339$\pm$9.4571\\                                                             % NOTINICML
S-SH3dmirror & 966.8579$\pm$9.6211\\                                                             % NOTINICML
lhs3dmirror & 1001.8826$\pm$9.2670\\                                                             % NOTINICML
sobol3dmirror & 1036.8494$\pm$10.1964\\                                                             % NOTINICML
naivedoe3dmirror & 1072.3794$\pm$11.1683\\                                                             % NOTINICML
Hammersley3dmirror & 1108.8699$\pm$10.7105\\                                                             % NOTINICML
random3dmirror & 1169.4045$\pm$12.2632\\                                                             % NOTINICML
Halton3dmirror & 1196.2969$\pm$11.4930\\                                                             % NOTINICML
	\hline                                                             % NOTINICML
	\end{tabular}                                                             % NOTINICML
  }}                                                             % NOTINICML
  \caption{\label{illcondcool}Minimum sampled objective function for the sphere function and for the illcond function (illcond has the most important variables first), but budget 37.}                                                             % NOTINICML
\end{table*}                                                             % NOTINICML
                                                             % NOTINICML
\subsection{Artificial xps on quasirandom, with most important variables last for illcond (reverseIllcond)}                                                             % NOTINICML
We recommended to use most critical variables first (section \ref{ordering});                                                              % NOTINICML
we here check results when the objective function is designed in a complete opposite manner, i.e.                                                              % NOTINICML
most important variables last - this is the case in which the user did not manage to properly rank the importance of variables.                                                              % NOTINICML
                                                             % NOTINICML
Consistently with theory, results (Table \ref{illcondnotcool}) for Halton and Hammersley are way worse than random at least in high dimension - whereas for illcond (previous section) Halton \& Hammersley were consistently better than random. On the other hand, scrambled variants and Sobol perform quite well - also consistently with theory as scrambling is aimed at improving results in high dimension.                                                             % NOTINICML
\begin{table*}\center                                                             % NOTINICML
{\scriptsize{                                                             % NOTINICML
\begin{tabular}{|c|c|}                                                             % NOTINICML
	\hline                                                             % NOTINICML
\multicolumn{2}{c}{Ranking in dimension 2}\\                                                             % NOTINICML
\hline                                                             % NOTINICML
S-SH & 0.0160$\pm$0.0003\\                                                             % NOTINICML
Hammersley & 0.0166$\pm$0.0004\\                                                             % NOTINICML
Halton & 0.0172$\pm$0.0004\\                                                             % NOTINICML
scr-Halton & 0.0175$\pm$0.0004\\                                                             % NOTINICML
scr-Halton3dmirror & 0.0186$\pm$0.0004\\                                                             % NOTINICML
naivedoe & 0.0219$\pm$0.0005\\                                                             % NOTINICML
sobol & 0.0220$\pm$0.0005\\                                                             % NOTINICML
naivedoe3dmirror & 0.0236$\pm$0.0006\\                                                             % NOTINICML
Hammersley3dmirror & 0.0240$\pm$0.0006\\                                                             % NOTINICML
random & 0.0241$\pm$0.0006\\                                                             % NOTINICML
lhs & 0.0247$\pm$0.0007\\                                                             % NOTINICML
S-SH3dmirror & 0.0250$\pm$0.0006\\                                                             % NOTINICML
random3dmirror & 0.0275$\pm$0.0007\\                                                             % NOTINICML
lhs3dmirror & 0.0278$\pm$0.0008\\                                                             % NOTINICML
Halton3dmirror & 0.0286$\pm$0.0007\\                                                             % NOTINICML
sobol3dmirror & 0.0306$\pm$0.0008\\                                                             % NOTINICML
\hline                                                             % NOTINICML
\multicolumn{2}{c}{Ranking in dimension 4}\\                                                             % NOTINICML
\hline                                                             % NOTINICML
Hammersley & 0.8421$\pm$0.0139\\                                                             % NOTINICML
S-SH & 0.8950$\pm$0.0148\\                                                             % NOTINICML
Halton & 0.9280$\pm$0.0168\\                                                             % NOTINICML
scr-Halton & 0.9343$\pm$0.0160\\                                                             % NOTINICML
sobol & 0.9534$\pm$0.0172\\                                                             % NOTINICML
lhs & 1.0184$\pm$0.0191\\                                                             % NOTINICML
naivedoe & 1.0913$\pm$0.0206\\                                                             % NOTINICML
S-SH3dmirror & 1.3770$\pm$0.0277\\                                                             % NOTINICML
sobol3dmirror & 1.4108$\pm$0.0275\\                                                             % NOTINICML
scr-Halton3dmirror & 1.5129$\pm$0.0376\\                                                             % NOTINICML
Hammersley3dmirror & 1.5228$\pm$0.0342\\                                                             % NOTINICML
random & 1.5522$\pm$0.0504\\                                                             % NOTINICML
lhs3dmirror & 1.6735$\pm$0.0336\\                                                             % NOTINICML
naivedoe3dmirror & 1.7350$\pm$0.0334\\                                                             % NOTINICML
Halton3dmirror & 1.9037$\pm$0.0581\\                                                             % NOTINICML
random3dmirror & 2.1842$\pm$0.0707\\                                                             % NOTINICML
\hline                                                             % NOTINICML
\end{tabular}                                                             % NOTINICML
\begin{tabular}{|c|c|}                                                             % NOTINICML
	\hline                                                             % NOTINICML
\multicolumn{2}{c}{Ranking in dimension 8}\\                                                             % NOTINICML
\hline                                                             % NOTINICML
sobol & 32.6119$\pm$0.3941\\                                                             % NOTINICML
naivedoe & 33.9010$\pm$0.4585\\                                                             % NOTINICML
lhs & 35.8900$\pm$0.4947\\                                                             % NOTINICML
S-SH & 36.0995$\pm$0.4765\\                                                             % NOTINICML
scr-Halton & 36.1118$\pm$0.4796\\                                                             % NOTINICML
random & 37.3243$\pm$0.5617\\                                                             % NOTINICML
Hammersley & 38.2483$\pm$0.5640\\                                                             % NOTINICML
Halton & 47.0927$\pm$0.7619\\                                                             % NOTINICML
lhs3dmirror & 59.1168$\pm$0.8528\\                                                             % NOTINICML
random3dmirror & 59.5059$\pm$0.8462\\                                                             % NOTINICML
scr-Halton3dmirror & 62.5933$\pm$0.9385\\                                                             % NOTINICML
S-SH3dmirror & 63.3482$\pm$1.0009\\                                                             % NOTINICML
sobol3dmirror & 64.7354$\pm$0.9509\\                                                             % NOTINICML
naivedoe3dmirror & 65.5584$\pm$0.8925\\                                                             % NOTINICML
Hammersley3dmirror & 78.7774$\pm$1.2885\\                                                             % NOTINICML
Halton3dmirror & 99.5334$\pm$1.7559\\                                                             % NOTINICML
\hline                                                             % NOTINICML
\multicolumn{2}{c}{Ranking in dimension 16}\\                                                             % NOTINICML
\hline                                                             % NOTINICML
S-SH & 902.1689$\pm$8.1918\\                                                             % NOTINICML
sobol & 926.6286$\pm$8.0765\\                                                             % NOTINICML
naivedoe & 938.6190$\pm$8.2898\\                                                             % NOTINICML
scr-Halton & 939.7127$\pm$8.8606\\                                                             % NOTINICML
lhs & 947.1720$\pm$9.0711\\                                                             % NOTINICML
random & 970.2377$\pm$9.5650\\                                                             % NOTINICML
scr-Halton3dmirror & 1323.8852$\pm$13.4973\\                                                             % NOTINICML
lhs3dmirror & 1350.1251$\pm$12.4491\\                                                             % NOTINICML
Hammersley & 1366.7788$\pm$15.4354\\                                                             % NOTINICML
sobol3dmirror & 1368.4549$\pm$12.4128\\                                                             % NOTINICML
S-SH3dmirror & 1369.0838$\pm$13.7944\\                                                             % NOTINICML
random3dmirror & 1369.8667$\pm$13.6301\\                                                             % NOTINICML
Halton & 1397.1004$\pm$15.9877\\                                                             % NOTINICML
naivedoe3dmirror & 1411.1522$\pm$14.8934\\                                                             % NOTINICML
Halton3dmirror & 1818.1474$\pm$19.1002\\                                                             % NOTINICML
Hammersley3dmirror & 1831.8963$\pm$20.3880\\                                                             % NOTINICML
\hline                                                             % NOTINICML
\end{tabular}                                                             % NOTINICML
}}                                                             % NOTINICML
\caption{\label{illcondnotcool}Best sampled point for the reverse illcond function, i.e. when most important variables are last - results are much worse, for quasirandom, that when they were ranked first. Smaller values for better results. Scrambled variants of Halton/Hammersley and Sobol resist much better than Halton/Hammersley. Mirrored samplers fail.}                                                             % NOTINICML
\end{table*}                                                             % NOTINICML
                                                             % NOTINICML
                                                             % NOTINICML
\subsection{Antisobol: a deceptive function for Sobol for one shot optimization}                                                             % NOTINICML
Table \ref{antisobol} presents results on the antisobol function, build as a deceptive function for the Sobol implementation we use - noticeably, results might depend on the direction vectors.                                                             % NOTINICML
HY refers to Hammersley, ND to Naive-Doe, S to Sobol, HN to Halton, SHN to Scrambled-Halton. The "S-" for random shift is discarded in this section and in the next section as all LDS in the present xps are randomly shifted. We see clearly disappointing results for Sobol, and excellent results for S-SH.                                                             % NOTINICML
\newcolumntype{H}{>{\setbox0=\hbox\bgroup}c<{\egroup}@{}}                                                             % NOTINICML
                                                             % NOTINICML
\begin{table*}                                                             % NOTINICML
	\center                                                             % NOTINICML
	\small                                                             % NOTINICML
	\begin{tabular}{ccccccccccccccccHHHHHHHHHHHHHHH}                                                             % NOTINICML
\hline                                                             % NOTINICML
	Dim & & & & & & & & & & & & & & & & & & & & & & & & & & & & & \\                                                             % NOTINICML
	\hline                                                             % NOTINICML
	2 & {\bf\em{R}} & HY & HY & SH & SH & SH & ND & SH & SH & HY & SH & HY & {\bf\em{R}} & SH & SH & SH & lhs & HY & SH & SH & HY & HY & HY & HY & HY & HY & SH & HY & SH & HY \\                                                             % NOTINICML
	3 & SH & SH & SH & HY & SH & SH & ND & ND & HY & SH & HY & SH & SH & ND & SH & lhs & SH & HY & SH & HY & ND & HY & SH & SH & lhs & SH & SH & SH & ND & SH \\                                                             % NOTINICML
	4 & SH & HY & lhs & HY & SH & HY & HY & {\bf\em{R}} & HY & HY & HY & SH & SH & HY & HY & SH & SH & HY & SH & HY & HY & lhs & HY & HY & HY & HY & SH & SH & lhs & SH \\                                                             % NOTINICML
	5 & SH & HY & lhs & HY & SH & HY & SH & ND & lhs & SH & HY & lhs & HY & HY & SH & HY & HY & SH & SH & HY & HY & HY & SH & SH & SH & SH & SH & HY & SH & HY \\                                                             % NOTINICML
	6 & SH & HY & {\bf\em{R}} & HY & SH & SH & HY & HY & SH & SH & HY & SH & SH & SH & SH & SH & HY & SH & {\bf\em{R}} & HY & lhs & SH & SH & HY & HY & HY & SH & HY & HY & HY \\                                                             % NOTINICML
	7 & SH & HY & HY & SH & SH & HY & SH & HY & {\bf\em{R}} & HY & SH & SH & HY & HY & HY & SH & HY & SH & SH & SH & HY & HY & HY & SH & HY & {\bf\em{R}} & HY & HY & HY & SH \\                                                             % NOTINICML
	8 & HY & HY & HY & HY & HY & ND & SH & SH & {\bf\em{R}} & SH & HY & SH & HY & HY & {\bf\em{R}} & {\bf\em{R}} & {\bf\em{R}} & SH & SH & HY & HY & HY & HY & HY & SH & {\bf\em{R}} & HY & HY & HY & HY \\                                                             % NOTINICML
	9 & SH & HY & SH & SH & SH & HY & SH & SH & lhs & HY & SH & SH & HY & SH & lhs & SH & HY & HY & SH & SH & {\bf\em{R}} & HY & SH & SH & HY & HY & SH & {\bf\em{R}} & SH & HY \\                                                             % NOTINICML
	\hline                                                             % NOTINICML
\end{tabular}                                                             % NOTINICML
                                                             % NOTINICML
	\begin{tabular}{cHHHHHHHHHHHHHHHccccccccccccccc}                                                             % NOTINICML
\hline                                                             % NOTINICML
	Dim & & & & & & & & & & & & & & & & & & & & & & & & & & & & & \\                                                             % NOTINICML
	\hline                                                             % NOTINICML
	2 & {\bf\em{R}} & HY & HY & SH & SH & SH & ND & SH & SH & HY & SH & HY & {\bf\em{R}} & SH & SH & SH & lhs & HY & SH & SH & HY & HY & HY & HY & HY & HY & SH & HY & SH & HY \\                                                             % NOTINICML
	3 & SH & SH & SH & HY & SH & SH & ND & ND & HY & SH & HY & SH & SH & ND & SH & lhs & SH & HY & SH & HY & ND & HY & SH & SH & lhs & SH & SH & SH & ND & SH \\                                                             % NOTINICML
	4 & SH & HY & lhs & HY & SH & HY & HY & {\bf\em{R}} & HY & HY & HY & SH & SH & HY & HY & SH & SH & HY & SH & HY & HY & lhs & HY & HY & HY & HY & SH & SH & lhs & SH \\                                                             % NOTINICML
	5 & SH & HY & lhs & HY & SH & HY & SH & ND & lhs & SH & HY & lhs & HY & HY & SH & HY & HY & SH & SH & HY & HY & HY & SH & SH & SH & SH & SH & HY & SH & HY \\                                                             % NOTINICML
	6 & SH & HY & {\bf\em{R}} & HY & SH & SH & HY & HY & SH & SH & HY & SH & SH & SH & SH & SH & HY & SH & {\bf\em{R}} & HY & lhs & SH & SH & HY & HY & HY & SH & HY & HY & HY \\                                                             % NOTINICML
	7 & SH & HY & HY & SH & SH & HY & SH & HY & {\bf\em{R}} & HY & SH & SH & HY & HY & HY & SH & HY & SH & SH & SH & HY & HY & HY & SH & HY & {\bf\em{R}} & HY & HY & HY & SH \\                                                             % NOTINICML
	8 & HY & HY & HY & HY & HY & ND & SH & SH & {\bf\em{R}} & SH & HY & SH & HY & HY & {\bf\em{R}} & {\bf\em{R}} & {\bf\em{R}} & SH & SH & HY & HY & HY & HY & HY & SH & {\bf\em{R}} & HY & HY & HY & HY \\                                                             % NOTINICML
	9 & SH & HY & SH & SH & SH & HY & SH & SH & lhs & HY & SH & SH & HY & SH & lhs & SH & HY & HY & SH & SH & {\bf\em{R}} & HY & SH & SH & HY & HY & SH & {\bf\em{R}} & SH & HY \\                                                             % NOTINICML
	\hline                                                             % NOTINICML
\end{tabular}                                                             % NOTINICML
                                                             % NOTINICML
                                                             % NOTINICML
                                                             % NOTINICML
	\caption{\label{antisobol}Best performing method, for each of 30 runs (one column per run), among the 8 presented methods, on the Antisobol function. Sobol performs poorly (never visible in the table), whereas random (R) is present several times. Randomly shifted scrambled Hammersley (denoted SH for short in the table) performs very well.}                                                             % NOTINICML
\end{table*}                                                             % NOTINICML
                                                             % NOTINICML
                                                             % NOTINICML
\subsection{Antish: Deceptive function for randomly shifted Scrambled-Hammersley}                                                             % NOTINICML
                                                             % NOTINICML
In Table \ref{antish}, dedicated to results on the Antish function made for being deceptive for S-SH, R wins 39 times, whereas SH wins 11 times and SHN wins 14 times; these scrambled variants of HN together win only 25 times - this shows that the Antish function is deceptive for S-SH and S-Halton.                                                              % NOTINICML
\begin{table*}\center                                                             % NOTINICML
	\scriptsize                                                             % NOTINICML
\begin{tabular}{ccccccccccccccccHHHHHHHHHHHHHHH}                                                             % NOTINICML
\hline                                                             % NOTINICML
	Dim & & & & & & & & & & & & & & & & & & & & & & & & & & & & & \\                                                             % NOTINICML
	\hline                                                             % NOTINICML
	12 & lhs & {\bf\em{R}} & {\bf\em{R}} & ND & lhs & ND & ND & S & ND & ND & ND & {\bf\em{R}} & {\bf\em{SH}} & {\bf\em{R}} & {\bf\em{R}} & {\bf\em{R}} & {\bf\em{R}} & S & lhs & S & lhs & lhs & {\bf\em{SHN}} & S & {\bf\em{R}} & {\bf\em{R}} & {\bf\em{R}} & S & lhs & {\bf\em{SH}} \\                                                             % NOTINICML
	13 & {\bf\em{SHN}} & S & lhs & {\bf\em{R}} & S & lhs & lhs & lhs & lhs & lhs & lhs & lhs & {\bf\em{R}} & S & ND & lhs & lhs & lhs & S & S & lhs & ND & {\bf\em{SH}} & S & {\bf\em{R}} & lhs & S & lhs & {\bf\em{SH}} & S \\                                                             % NOTINICML
	14 & lhs & {\bf\em{R}} & S & S & lhs & S & {\bf\em{R}} & S & ND & lhs & S & lhs & {\bf\em{SH}} & {\bf\em{R}} & S & ND & S & ND & ND & {\bf\em{R}} & lhs & S & {\bf\em{R}} & {\bf\em{R}} & ND & {\bf\em{SHN}} & lhs & lhs & S & S \\                                                             % NOTINICML
	15 & S & lhs & ND & ND & lhs & ND & lhs & lhs & lhs & lhs & S & lhs & ND & S & ND & S & S & {\bf\em{R}} & {\bf\em{R}} & {\bf\em{SH}} & lhs & {\bf\em{R}} & {\bf\em{R}} & S & S & S & {\bf\em{SHN}} & {\bf\em{R}} & lhs & {\bf\em{SH}} \\                                                             % NOTINICML
	16 & ND & {\bf\em{SH}} & {\bf\em{SHN}} & S & ND & {\bf\em{R}} & ND & ND & ND & lhs & lhs & ND & {\bf\em{R}} & ND & ND & ND & S & ND & {\bf\em{SHN}} & {\bf\em{SH}} & {\bf\em{R}} & S & S & {\bf\em{R}} & ND & S & {\bf\em{SHN}} & lhs & lhs & lhs \\                                                             % NOTINICML
	17 & lhs & S & lhs & S & ND & {\bf\em{R}} & lhs & S & S & S & ND & lhs & {\bf\em{SHN}} & lhs & lhs & {\bf\em{SH}} & {\bf\em{SHN}} & S & S & {\bf\em{R}} & S & ND & lhs & {\bf\em{SHN}} & {\bf\em{R}} & {\bf\em{R}} & lhs & S & ND & {\bf\em{R}} \\                                                             % NOTINICML
	18 & {\bf\em{R}} & ND & ND & S & S & {\bf\em{R}} & {\bf\em{R}} & ND & {\bf\em{R}} & ND & lhs & ND & {\bf\em{SHN}} & ND & S & S & S & lhs & {\bf\em{SHN}} & {\bf\em{R}} & S & {\bf\em{R}} & {\bf\em{SHN}} & {\bf\em{SHN}} & lhs & ND & lhs & lhs & lhs & {\bf\em{SH}} \\                                                             % NOTINICML
	\hline                                                             % NOTINICML
\end{tabular}                                                             % NOTINICML
\begin{tabular}{cHHHHHHHHHHHHHHHccccccccccccccc}                                                             % NOTINICML
\hline                                                             % NOTINICML
	Dim & & & & & & & & & & & & & & & & & & & & & & & & & & & & & \\                                                             % NOTINICML
	\hline                                                             % NOTINICML
	12 & lhs & {\bf\em{R}} & {\bf\em{R}} & ND & lhs & ND & ND & S & ND & ND & ND & {\bf\em{R}} & {\bf\em{SH}} & {\bf\em{R}} & {\bf\em{R}} & {\bf\em{R}} & {\bf\em{R}} & S & lhs & S & lhs & lhs & {\bf\em{SHN}} & S & {\bf\em{R}} & {\bf\em{R}} & {\bf\em{R}} & S & lhs & {\bf\em{SH}} \\                                                             % NOTINICML
	13 & {\bf\em{SHN}} & S & lhs & {\bf\em{R}} & S & lhs & lhs & lhs & lhs & lhs & lhs & lhs & {\bf\em{R}} & S & ND & lhs & lhs & lhs & S & S & lhs & ND & {\bf\em{SH}} & S & {\bf\em{R}} & lhs & S & lhs & {\bf\em{SH}} & S \\                                                             % NOTINICML
	14 & lhs & {\bf\em{R}} & S & S & lhs & S & {\bf\em{R}} & S & ND & lhs & S & lhs & {\bf\em{SH}} & {\bf\em{R}} & S & ND & S & ND & ND & {\bf\em{R}} & lhs & S & {\bf\em{R}} & {\bf\em{R}} & ND & {\bf\em{SHN}} & lhs & lhs & S & S \\                                                             % NOTINICML
	15 & S & lhs & ND & ND & lhs & ND & lhs & lhs & lhs & lhs & S & lhs & ND & S & ND & S & S & {\bf\em{R}} & {\bf\em{R}} & {\bf\em{SH}} & lhs & {\bf\em{R}} & {\bf\em{R}} & S & S & S & {\bf\em{SHN}} & {\bf\em{R}} & lhs & {\bf\em{SH}} \\                                                             % NOTINICML
	16 & ND & {\bf\em{SH}} & {\bf\em{SHN}} & S & ND & {\bf\em{R}} & ND & ND & ND & lhs & lhs & ND & {\bf\em{R}} & ND & ND & ND & S & ND & {\bf\em{SHN}} & {\bf\em{SH}} & {\bf\em{R}} & S & S & {\bf\em{R}} & ND & S & {\bf\em{SHN}} & lhs & lhs & lhs \\                                                             % NOTINICML
	17 & lhs & S & lhs & S & ND & {\bf\em{R}} & lhs & S & S & S & ND & lhs & {\bf\em{SHN}} & lhs & lhs & {\bf\em{SH}} & {\bf\em{SHN}} & S & S & {\bf\em{R}} & S & ND & lhs & {\bf\em{SHN}} & {\bf\em{R}} & {\bf\em{R}} & lhs & S & ND & {\bf\em{R}} \\                                                             % NOTINICML
	18 & {\bf\em{R}} & ND & ND & S & S & {\bf\em{R}} & {\bf\em{R}} & ND & {\bf\em{R}} & ND & lhs & ND & {\bf\em{SHN}} & ND & S & S & S & lhs & {\bf\em{SHN}} & {\bf\em{R}} & S & {\bf\em{R}} & {\bf\em{SHN}} & {\bf\em{SHN}} & lhs & ND & lhs & lhs & lhs & {\bf\em{SH}} \\                                                             % NOTINICML
	\hline                                                             % NOTINICML
\end{tabular}                                                             % NOTINICML
	\caption{\label{antish}Best method for different runs of different dimensions, on the AntiSh function designed for being deceptive for the randomly shifted Scrambled Hammersley. Each column corresponds to one of 30 runs, each row corresponds to a different dimensionality. Each cell shows which method performed best. Random performed well overall, but the gap with randomly shifted scrambled Hammersley (denoted SH in the present table) is small, whereas in Fig. \ref{antisobol} we could exhibit a function for which Sobol performed very poorly - it seems easier to find counterexamples for Sobol than for SH (at least, for the version of Sobol we use, and for SH with random scrambling and randomly shifted).}                                                             % NOTINICML
\end{table*}                                                             % NOTINICML
